# Supplementary material for: Monotonic Cardinality Estimation of Similarity Selection: A Deep Learning Approach
Source: arXiv:2002.06442 source file (2021-09-24)
Supplement: Supplementary file 1 [file appendix.tex]

\section{Proofs} \label{sec:proof}

\subsection{Lemma~\ref{lm:overall-monotonicity}}
\begin{proof}
  Consider two queries $(x, \theta_1)$ and $(x, \theta_2)$, where $\theta_1 \leq \theta_2$.
  $(\mathbf{x}, \tau_1) = h(x, \theta_1)$ and $(\mathbf{x}, \tau_2) = h(x, \theta_2)$. 
  Because $h(x, \theta)$ is monotonically increasing with $\theta$, $\tau_1 \leq \tau_2$. 
  Because $g(\mathbf{x}, \tau)$ is monotonically increasing with $\tau$, $g(\mathbf{x}, \tau_1) 
  \leq g(\mathbf{x}, \tau_2)$. Because $g \circ h(x, \theta_1) = g(\mathbf{x}, \tau_1)$ 
  and $g \circ h(x, \theta_2) = g(\mathbf{x}, \tau_2)$, 
  $g \circ h(x, \theta_1) \leq g \circ h(x, \theta_2)$. The monotonicity is proved. 
\end{proof}

\subsection{Lemma~\ref{lm:model-monotonicity}}
\begin{proof}
  Consider $\pair{\mathbf{x}, \tau_1}$ and $\pair{\mathbf{x}, \tau_2}$, and $\tau_1 \leq \tau_2$.
  %$g(\mathbf{x}, \tau_2) - g(\mathbf{x}, \tau_1) = \sum_{i=\tau_1 + 1}^{\tau_2}{\textsf{ReLU}(\mathbf{w}_i^{\rm T}\Psi(\mathbf{x}) + b_i)}$. 
  Because $g_i$ is deterministic, 
  $g(\mathbf{x}, \tau_2) - g(\mathbf{x}, \tau_1) = \sum_{i=\tau_1 + 1}^{\tau_2}{g_i(\mathbf{x})}$. 
  Because $g_i$ is non-negative, $\sum_{i=\tau_1 + 1}^{\tau_2}{g_i(\mathbf{x})} \geq 0$. 
  Thus, $g(\mathbf{x}, \tau)$ is monotonically increasing with $\tau$.
\end{proof}

\section{Experiment Setup Details} 

\subsection{Parameter Settings} \label{sec:parameter}
%\myparagraph{Parameter Settings} 
\textit{Feature extraction}: we use 256 hash functions for Jaccard 
distance, 256 (on \gloveone) and 512 (on \glovetwo) hash functions %($r = 0.05$) 
for Euclidean distance. 

\textit{Hyperparameters}: The \vae a fully-connected neural network, with three hidden 
layers of 256, 128, and 128 nodes for both encoder and decoder. The activation function 
is \textsf{ELU}, in line with \cite{kingma2013auto}. The dimensionality of the \vae's 
output is 40, 60, 128, 128, 128, 64, 64, 64, 64, 128, as per the order in 
Table~\ref{tab:dataset}. For both $\Phi$ (\modelone) and $\Phi'$ (\modeltwo), we use a 
fully-connected neural network with four hidden layers of 512, 512, 256, and 256 nodes. 
The activation function is \textsf{ReLU}. The dimensionality of distance embeddings is 5. 
The dimensionality of final embeddings $\mathbf{z}_x^i$ is 60. 
We set $\lambda$ in Equation~\ref{eq:monomodel1:loss} and $\lambda_{\Delta}$ in 
Equation~\ref{eq:monomodel1:lossnn} to both 0.1. 
%\warn{which aims to make sure
%that \vae and dynamic training do not dominate the overrall training procedure.}

% For threshold
% embedding in \modelone, we use 5 
% dimensional embedding vector. The dimension of dense representation of
% our \vae used in the experiment is 40 for 64-bits data and 80
% for 128-bits data and 128 for string-based data.
%To train our model, we adopt to achieve
%relatively good performance in testing data. 
% For the other hyperparameters (e.g., the dimensionality of $\mathbf{z}^i_x$), 
% we fine-tune the entire network using the training and validation dataset. 
\textit{Training}: We first train \vae for 100 epochs. To train \modelone and 
\modeltwo, we use stochastic gradient descent and set the initial learning rate 
as 0.001. The regression model is first trained with the basic loss function 
$\mathcal{L}_{g} = \msle$ for 500 epochs. Then we reset the learning rate as 
0.00025 and decrease its value per epoch with decay of learning rate 
$\gamma = 5 \cdot 10^{-4}$. Then the regression model is trained with the loss 
function in Equation~\ref{eq:monomodel1:lossnn} for another 300 epochs. 
Validation is performed every 10 epochs. Finally, the one with the smallest 
validation error is selected for the evaluation on testing data. 

\subsection{Experimental Environment} \label{sec:environment}
%\myparagraph{Environments}
The experiments were carried out on a server with a Intel Xeon E5-2640 @2.40GHz 
Processor, GPU GeForce GTX 1080 Ti, and 256GB RAM running Ubuntu 16.04.4 LTS. 
Non-deep models were implemented in C++. Deep models were trained in Tensorflow, 
and then the parameters were copied to C++ implementations for a fair comparison 
of estimation efficiency. 
% We implemented deep models in TensorFlow, database methods 
% in C++, \kdeexp in Java, and \xgbexp in Python using the XGBoost library~\cite{URL:xgboost}. 

\section{Additional Experiments} \label{sec:additional-exp}

\subsection{Monotonicity Test}

\begin{table} [t]
  \small%\scriptsize
  \caption{Monotonicity test (\textsf{DgrMon}, \%).}
  \label{tab:monotest}
  \centering
  \begin{tabular}[t]{| l | c | c | c | c |}
    \hline%
    Model & \pubchem & \dblped & \bmsjacc & \gloveone\\
    \hline%
    \spestexp & 100.0 & 100.0 & 100.0 & 100.0 \\
    %\hline%
    \usexp & 100.0 & 100.0 & 100.0 & 100.0 \\
    %\hline%    
    \xgbexp & 60.0 & 46.0 & 74.6 & 81.3 \\ 
    %\hline%
    \lightgbmexp & x.x & x.x & x.x & x.x \\
    %\hline%
    \kdeexp & 100.0 & 100.0 & 100.0 & 100.0 \\
    %\hline%
    \dlnexp & 100.0 & 100.0 & 100.0 & 100.0\\ 
    %\hline% 
    \moeexp & 75.7 & 57.7 & 53.1 & 86.4 \\
    %\hline%
    \hierdnnexp & 93.7 & 87.4 & 65.4 & 93.6 \\
    %\hline%    
    \dnnexp & 88.5 & 63.4 & 76.8 & 93.6 \\
    %\hline% 
    \dnnsexp & 69.1 & 58.2 & 48.7 & 68.6 \\  
    %\hline%
    %\textsf{MonoNet} & 100.00 & 100.00 & 100.00 & 100.00 & 100.00\\
    %\hline%
    %\hline%
    \lstmexp & - & x.x & - & - \\
    %\hline% 
    \lstmaexp & - & x.x & - & - \\     
    \textbf{\modelone} & 100.0 & 100.0 & 100.0 & 100.0\\
    %\hline%
    \textbf{\modeltwo} & 100.0 & 100.0 & 100.0 & 100.0\\
    \hline%
  \end{tabular}
\end{table}

In Table~\ref{tab:monotest}, we evaluate the monotonicity 
by measuring degree of monotonicity (\textsf{DgrMon})~\cite{daniels2010monotone}: 
%\begin{align*}
  $\textsf{DgrMon} = \frac{\text{\# monotonic pairs}(\mathcal{P})}{\text{\# comparable pairs}(\mathcal{P})}$, 
%\end{align*}
where $\mathcal{P}$ is the set of data pairs to test. 
We uniformly sample 100 query records, and 
enumerate all the thresholds $0, 1, \dots, \theta_{max}$ for each query record. 
Given a query $x$ and two thresholds $\theta$ and $\theta + 1$, 
a pair is generated as $\pair{\widehat{c}_{\theta}, \widehat{c}_{\theta + 1}}$, 
where $0 \leq \theta < \theta_{max}$, and $\widehat{c}_{\theta}$ is the cardinality 
of $x$ with threshold $\theta$. 
If a pair is monotonic, then $\widehat{c}_{\theta} \leq \widehat{c}_{\theta + 1}$. 
The results are shown in Table~\ref{tab:monotest}. 
Database methods, \kdeexp, \dlnexp, and our models are monotonic on all the pairs 
(100\% \textsf{DgrMon}). \kdeexp considers 
the distances between the query and the samples in metric space, so it guarantees the 
monotonicity. Database methods can achieve monotonicity by carefully selecting samples 
with different thresholds. Among all the other models, \hierdnnexp achieves high 
percentage of monotonicity. E.g., its \textsf{DgrMon}s are larger than 90\% on \pubchem 
and \gloveone. 
This indicates its strategy of partitioning output space can preserve
some monotonicity. 
\moeexp does not have very good monotonicity performance, because its strategy assigns
inputs to proper experts but does not consider any monotonicity. Our models guarantee 
the monotinicity and the experiment confirms this.

\begin{table*} [t]
  \small%\scriptsize
  \caption{Model size (MB).}
  \label{tab:modelsize}
  \centering
  \begin{tabular}[b]{| l | c | c | c | c | c | c | c | c |}
    \hline%
    Model & \imagenet & \pubchem & \aminer & \dblped & \bmsjacc & \dblpjacclong & \gloveone & \glovetwo \\
    \hline%
    \spestexp & 10.4 & 143.2 & 31.2 & 142.4 & 39.4 & 74.5 & 86.5 & 86.2 \\
    %\hline%
    \usexp & 0.6 & 2.6 & 0.5 & 0.7 & 0.6 & 0.7 & 1.2 & 3.4 \\
    %\hline%    
    %\textsf{EnsembleSVM} &  &  &  & & \\
    %\hline%
    %\textsf{C-SVR} & 45 & 637 & 74 & & \\
    %\hline%
    %\textsf{RFR} & 48 & 97 & 105 & & \\
    %\hline%
    %\textsf{C-RFR} & 34 & 113 & 109 & & \\
    %\hline%
    \xgbexp & 36.4 & 68.2 & 36.4 & 48.5 & 48.8 & 63.2 & 63.2 & 63.2 \\
    %\hline%
    \lightgbmexp & x.x & x.x & x.x & x.x & x.x & x.x & x.x & x.x \\
    %\hline%
    \kdeexp & 4.5 & 8.4 & 1.5 & 7.1 & 3.6 & 7.5 & 7.7 & 18.1 \\
    %\hline%
    \dlnexp & 28.4 & 76.6 & 75.4 & 186.8 & 28.6 & 38.2 & 26.6 & 64.4 \\
    %\hline%    
    \moeexp & 16.8 & 40.5 & 52.5 & 101.2 & 35.4 & 48.5 & 36.9 & 52.5 \\
    %\hline%
    \hierdnnexp & 57.7 & 80.4 & 84.8 & 122.5 & 54.6 & 65.4 & 60.6 & 66.1 \\
    %\hline%
    \dnnexp & 5.0 & 11.4 & 14.5 & 49.7 & 8.7 & 7.4 & 6.3 & 9.8 \\
    %\hline%    
    \dnnsexp & 105.4 & 337.3 & 154.2 & 485.0 & 183.2 & 382.7 & 132.0 & 158.4 \\
    %\hline%
    %\textsf{MonoNet} & & & & & \\
    %\hline%
    %\hline%
    \textbf{\modelone} & 9.6 & 38.5 & 40.2 & 96.2 & 16.4 & 19.7 & 21.2 & 23.8 \\
    %\hline%
    \textbf{\modeltwo} & 16.2 & 46.3 & 54.5 & 105.1 & 22.8 & 25.3 & 31.2 & 35.3 \\
    \hline%
  \end{tabular}
\end{table*}

\subsection{Model Size}
Table~\ref{tab:modelsize} shows the storage sizes of the competitors. \usexp does not 
need any storage and thus shows zero model size. \kdeexp achieves the smallest model size 
among others, because it only needs to store the kernel instances to assist estimation. For 
deep models, \dnnexp has the smallest model size. Our model size ranges from 10 to 105 MB. 
It is at most 3 times larger than \dnnexp and smaller than the other deep models. 
Considering the significant improvement of accuracy, the storage of our models is acceptable. 

\subsection{Evaluation of Training}

\subsubsection{Training Time}
Compare training time with other methods. 

\subsubsection{Varying the Size of Training Data}

\begin{table} [t]
  \small%\scriptsize
  \caption{Accuracy v.s. training examples.}
  \label{tab:trainnum}
  \centering
  \begin{tabular}[b]{| l | l | c | c | c | c | c |}
    \hline%
    Metric & Dataset & 20\% & 40\% & 60\% & 80\%
    & 100\% \\
    \hline%
    \multirow{4}{*}{\textsf{MSE}} &
    \imagenet & 4373 & 3486 & 3181 & 3096 & 3044\\ 
    %\hline%
    & \aminer & 91429 & 76647 & 73438 & 69130 & 64831 \\
    %  %\hline%
    % & \bmsoverlap & 766145 & 352071 & 275118 & 217382 & 156365 \\
    %  %\hline% 
    & \bmsjacc & 107 & 89 & 87 & 71 & 64 \\  
    % \hline%
    & \glovetwo & 20770 & 18115 & 9109 & 15848 & 16809 \\
    %\hline%
    \hline%
    \hline%    
    \multirow{4}{*}{\textsf{MAPE}} &
    \imagenet & 11.65 & 10.98 & 10.40 & 9.71 & 9.63 \\ 
    %\hline%
    & \aminer & 53.11 & 50.22 & 47.83 & 46.14 & 44.78 \\
     %\hline%
    % & \bmsoverlap & 14.83 & 12.73  & 11.99 & 11.71 & 11.40 \\
    %  %\hline% 
    & \bmsjacc & 20.32 & 17.81 & 12.25 & 13.19 & 13.94 \\  
     %\hline%
    & \glovetwo & 6.99 & 5.62 & 4.16 & 4.62 & 4.58 \\
    \hline%
  \end{tabular}
\end{table}
In Table~\ref{tab:trainnum}, we show the performance of \modeltwo by varying the number 
of training examples. We use one dataset for each distance function, and randomly sample 
20\%, 40\%, 60\%, and 80\% training data to separately train our model. 
The experimental results show that our model
is robust with the training data size and has enough capability to generalize well. 
E.g., on \imagenet, the \mse and \mape of our model only increase to 1.4 and 1.2 times, 
respectively, when the number of training data are reduced by 80\%.~\findme{We need a set 
of 8 figures for this experiment. See the experiments on varying training datas in Anhai 
Doan's SIGMOD 2018 paper.}
% For example, in \imagenet, the gap of 20\% and 100\% training data 
% (1.44 times for \mse and 1.21 times for \mape) is not large. 

\begin{figure} [t]
  \centering
  \subfigure[\textsf{MSE}, \imagenet]{
    \includegraphics[width=0.46\linewidth]{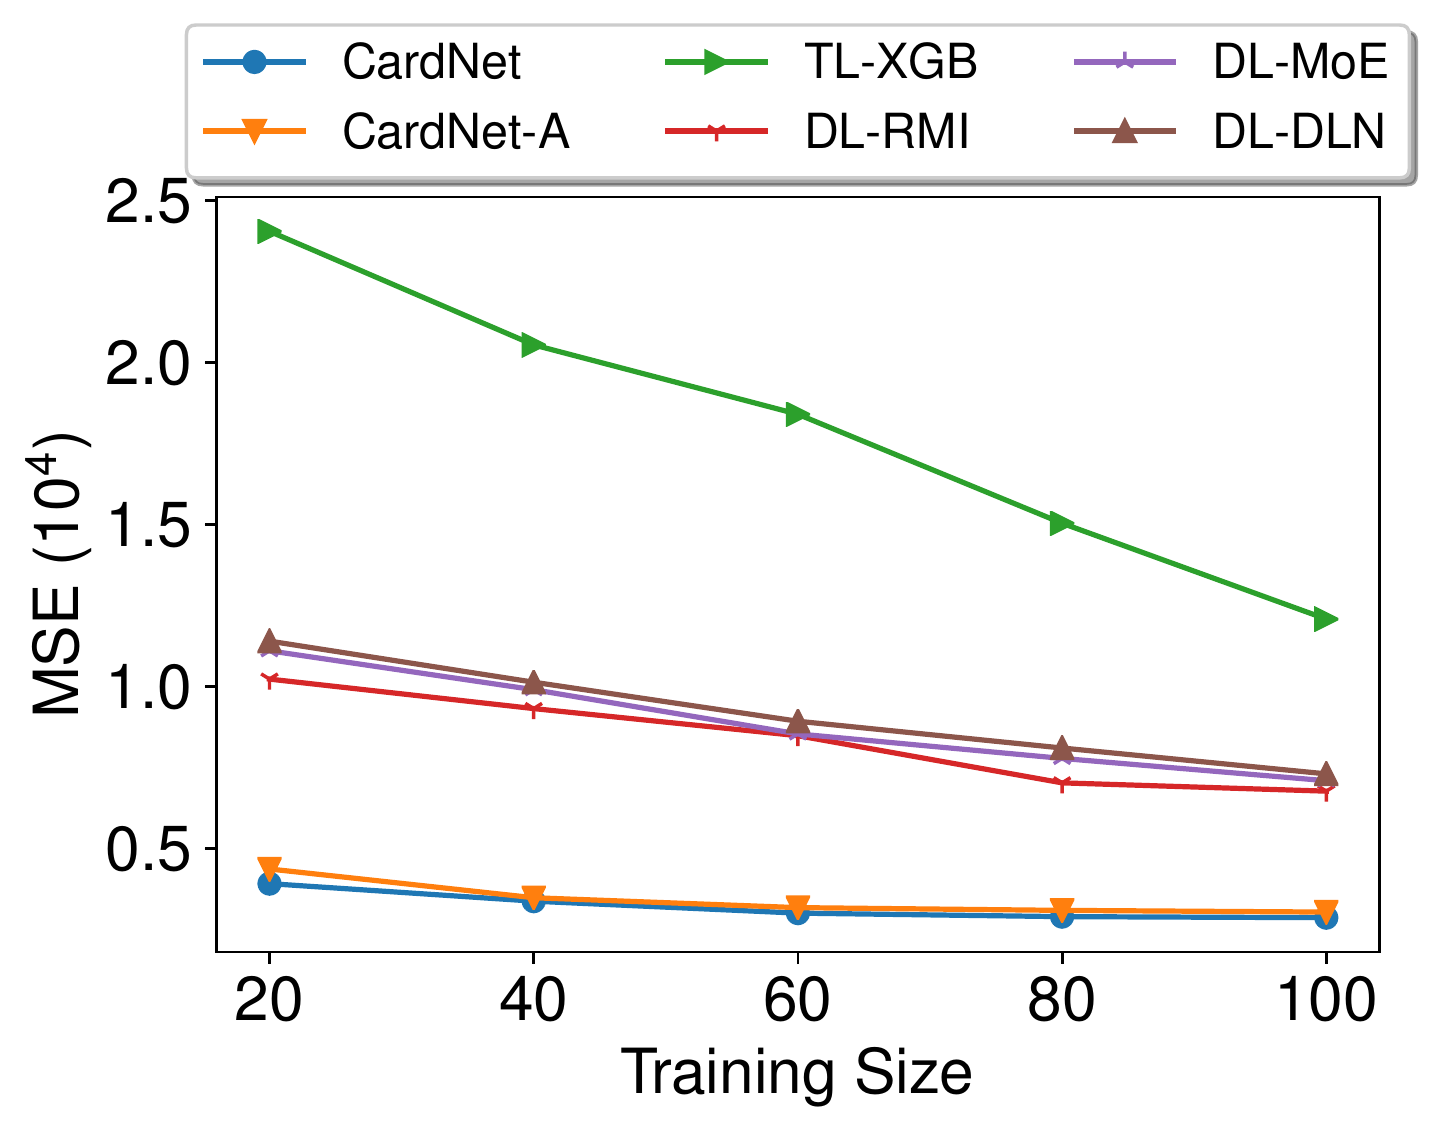}
    \label{fig:exp-imagenet-mse-trainsize}
  }
  \subfigure[\textsf{MAPE}, \imagenet]{
    \includegraphics[width=0.46\linewidth]{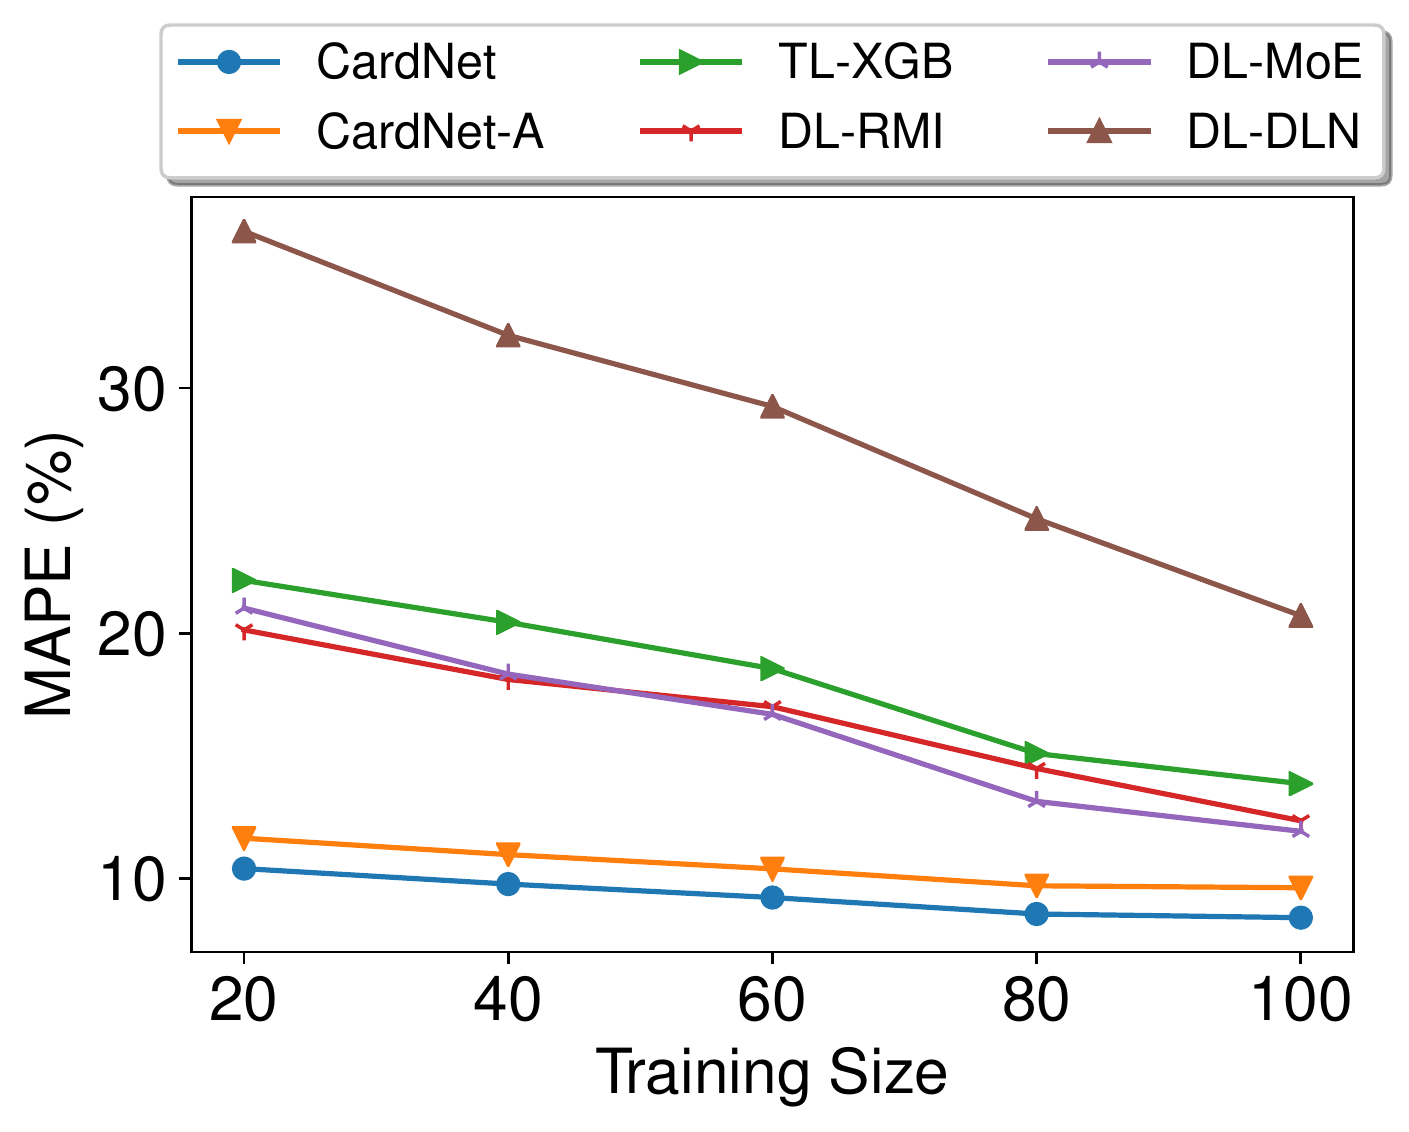}
    \label{fig:exp-imagenet-mape-trainsize}
  }
  \subfigure[\textsf{MSE}, \aminer]{
    \includegraphics[width=0.46\linewidth]{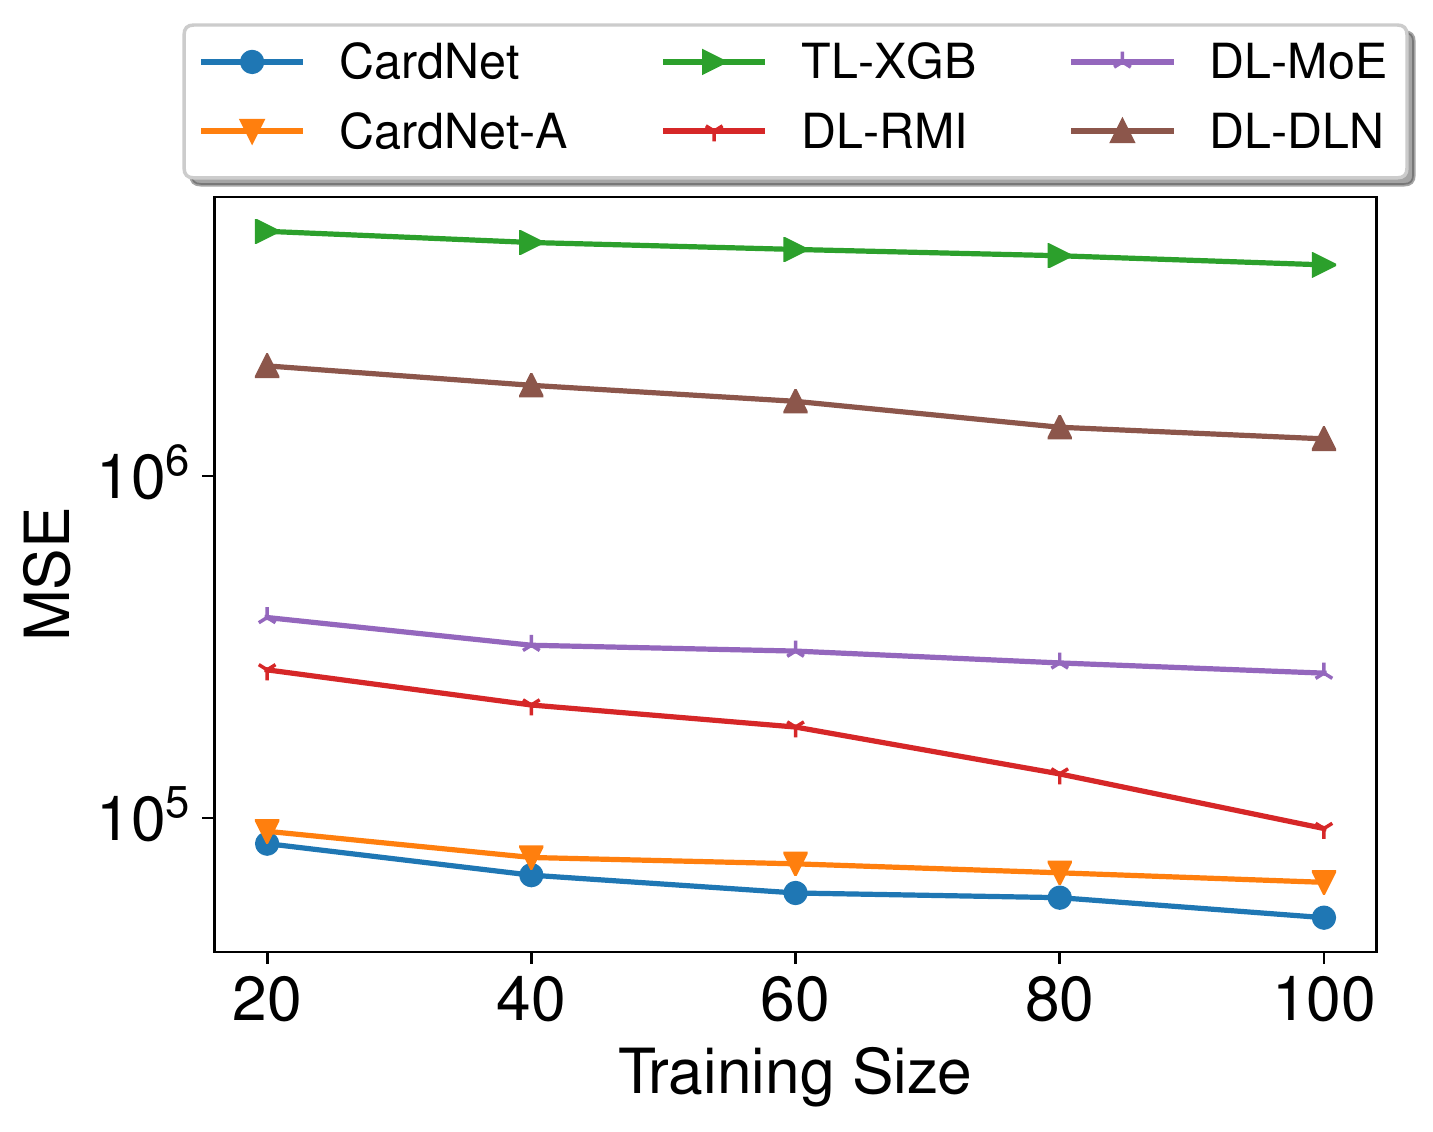}
    \label{fig:exp-aminer-mse-trainsize}
  }
  \subfigure[\textsf{MAPE}, \aminer]{
    \includegraphics[width=0.46\linewidth]{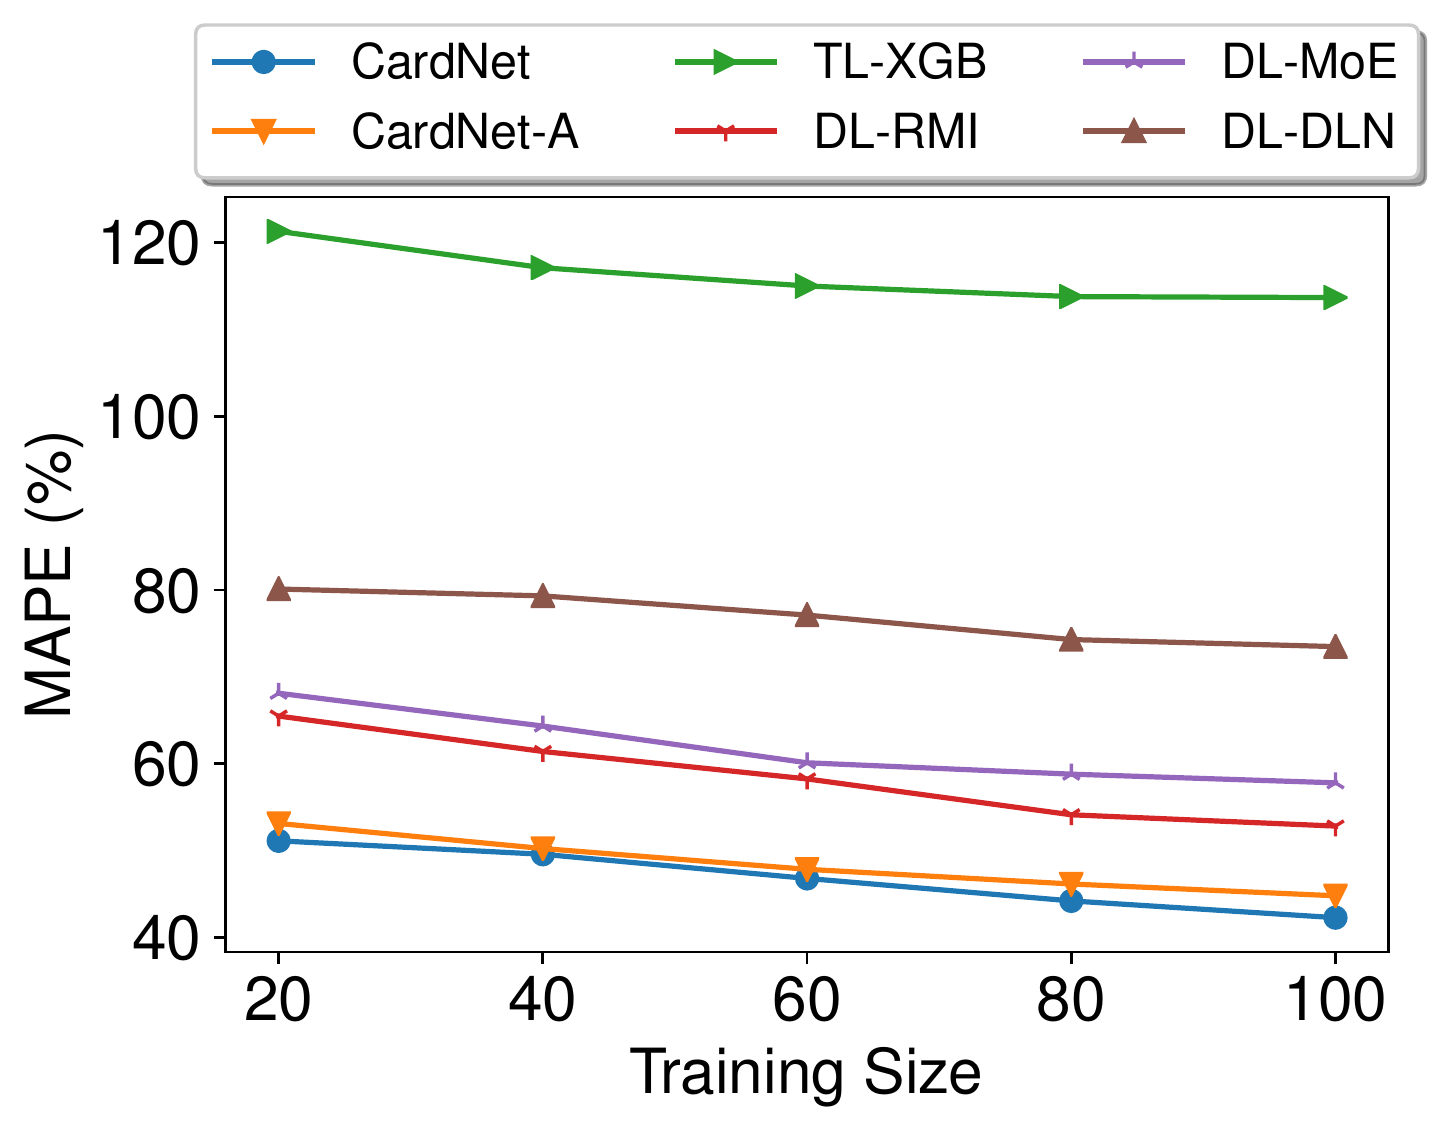}
    \label{fig:exp-aminer-mape-trainsize}
  }
  \subfigure[\textsf{MSE}, \bmsjacc]{
    \includegraphics[width=0.46\linewidth]{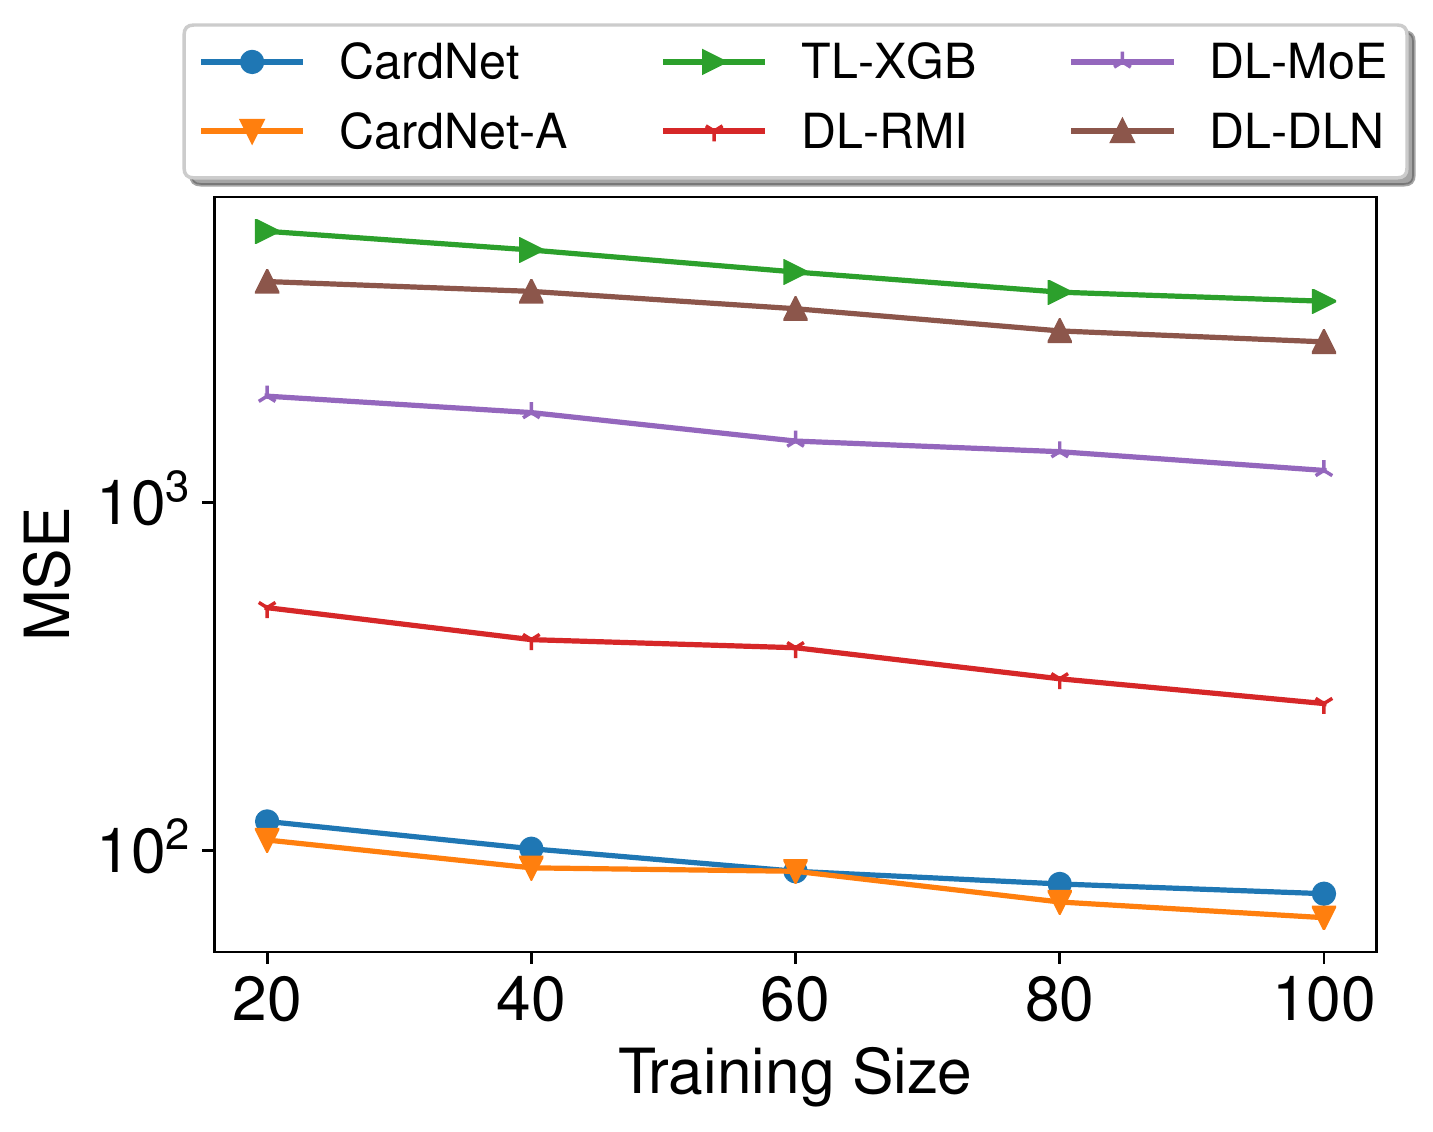}
    \label{fig:exp-bms-mse-trainsize}
  }
  \subfigure[\textsf{MAPE}, \bmsjacc]{
    \includegraphics[width=0.46\linewidth]{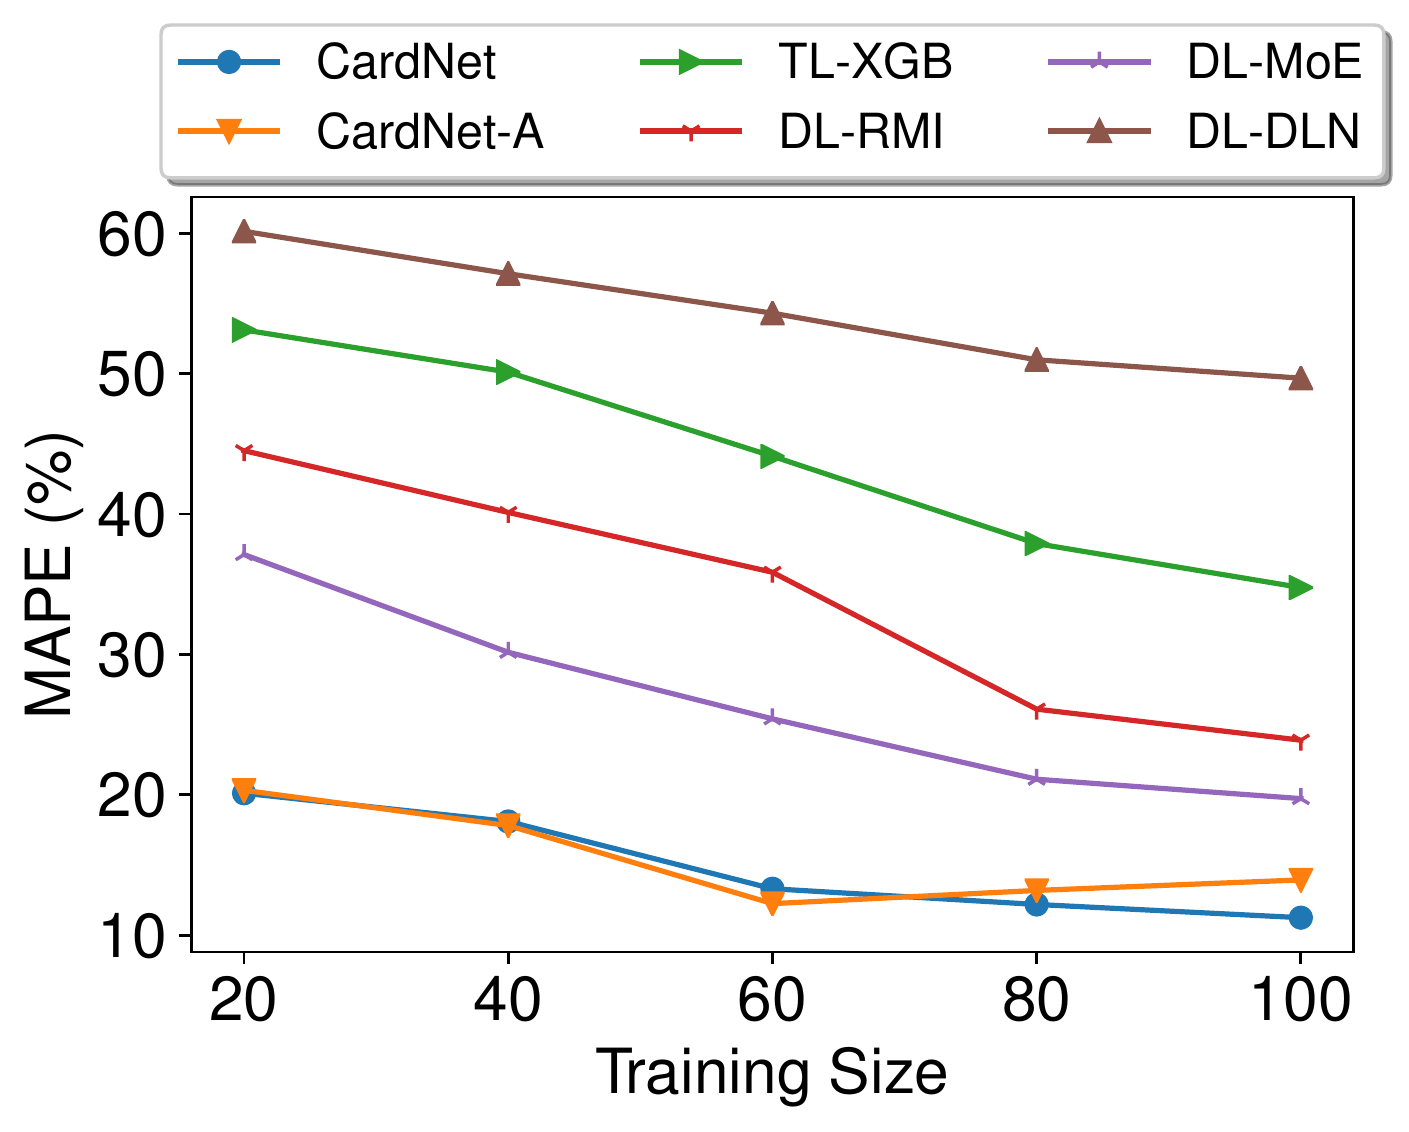}
    \label{fig:exp-bms-mape-trainsize}
  }
  \subfigure[\textsf{MSE}, \glovetwo]{
    \includegraphics[width=0.46\linewidth]{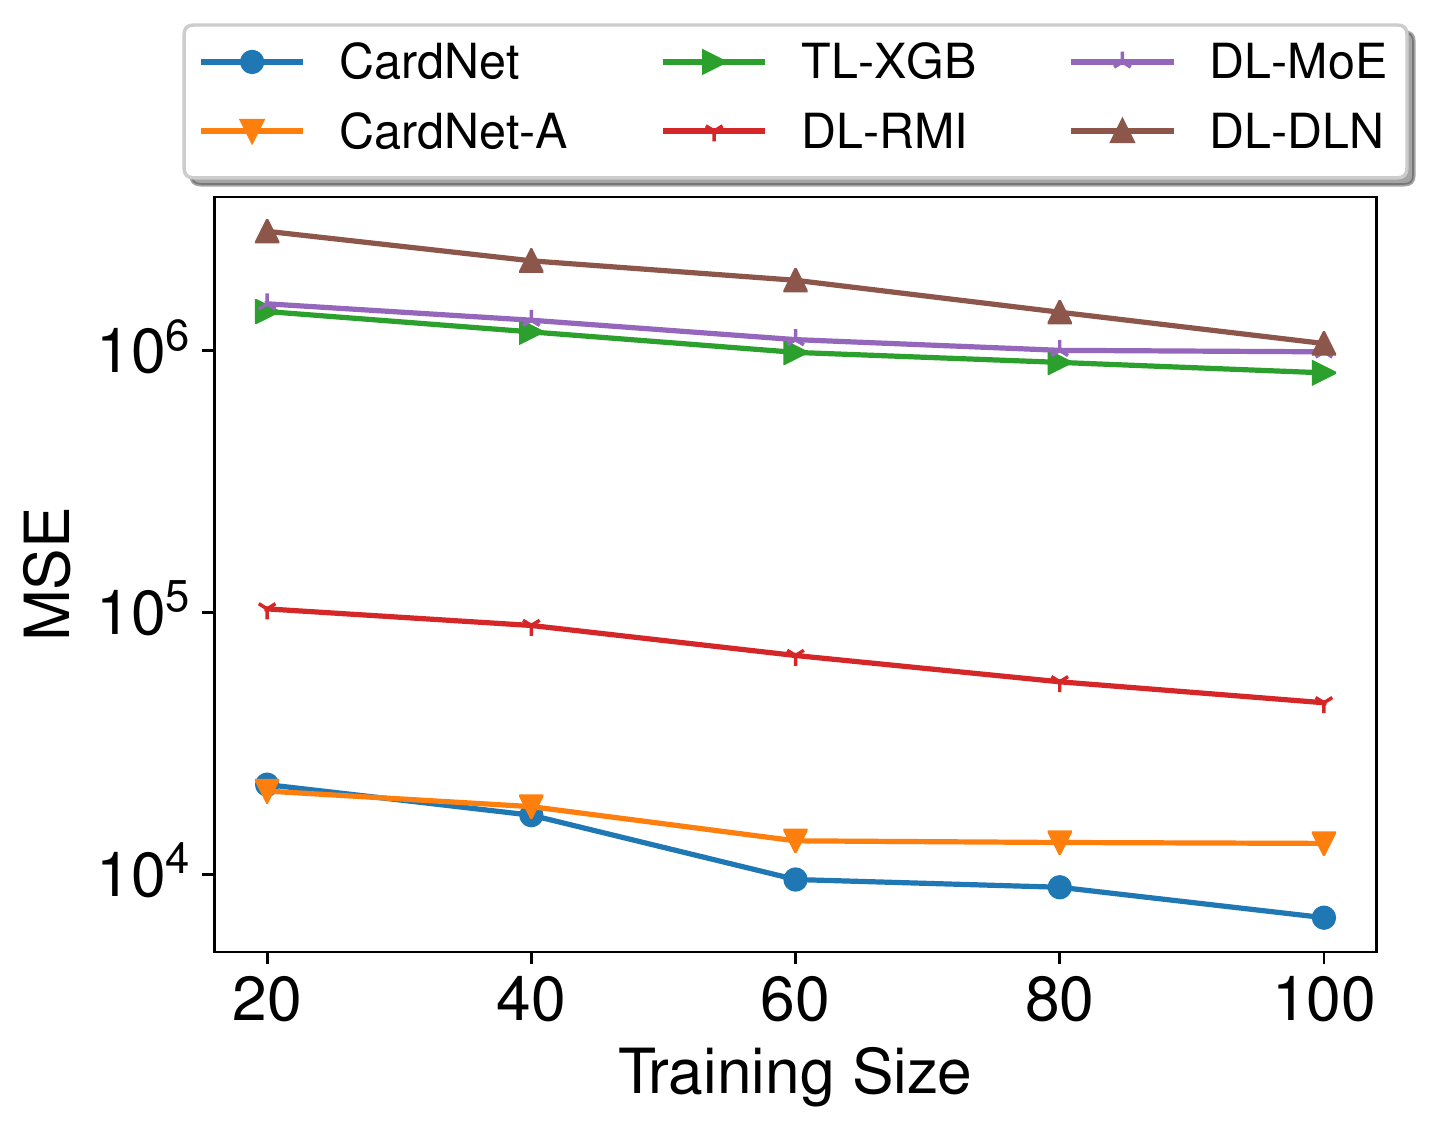}
    \label{fig:exp-glove-mse-trainsize}
  }
  \subfigure[\textsf{MAPE}, \glovetwo]{
    \includegraphics[width=0.46\linewidth]{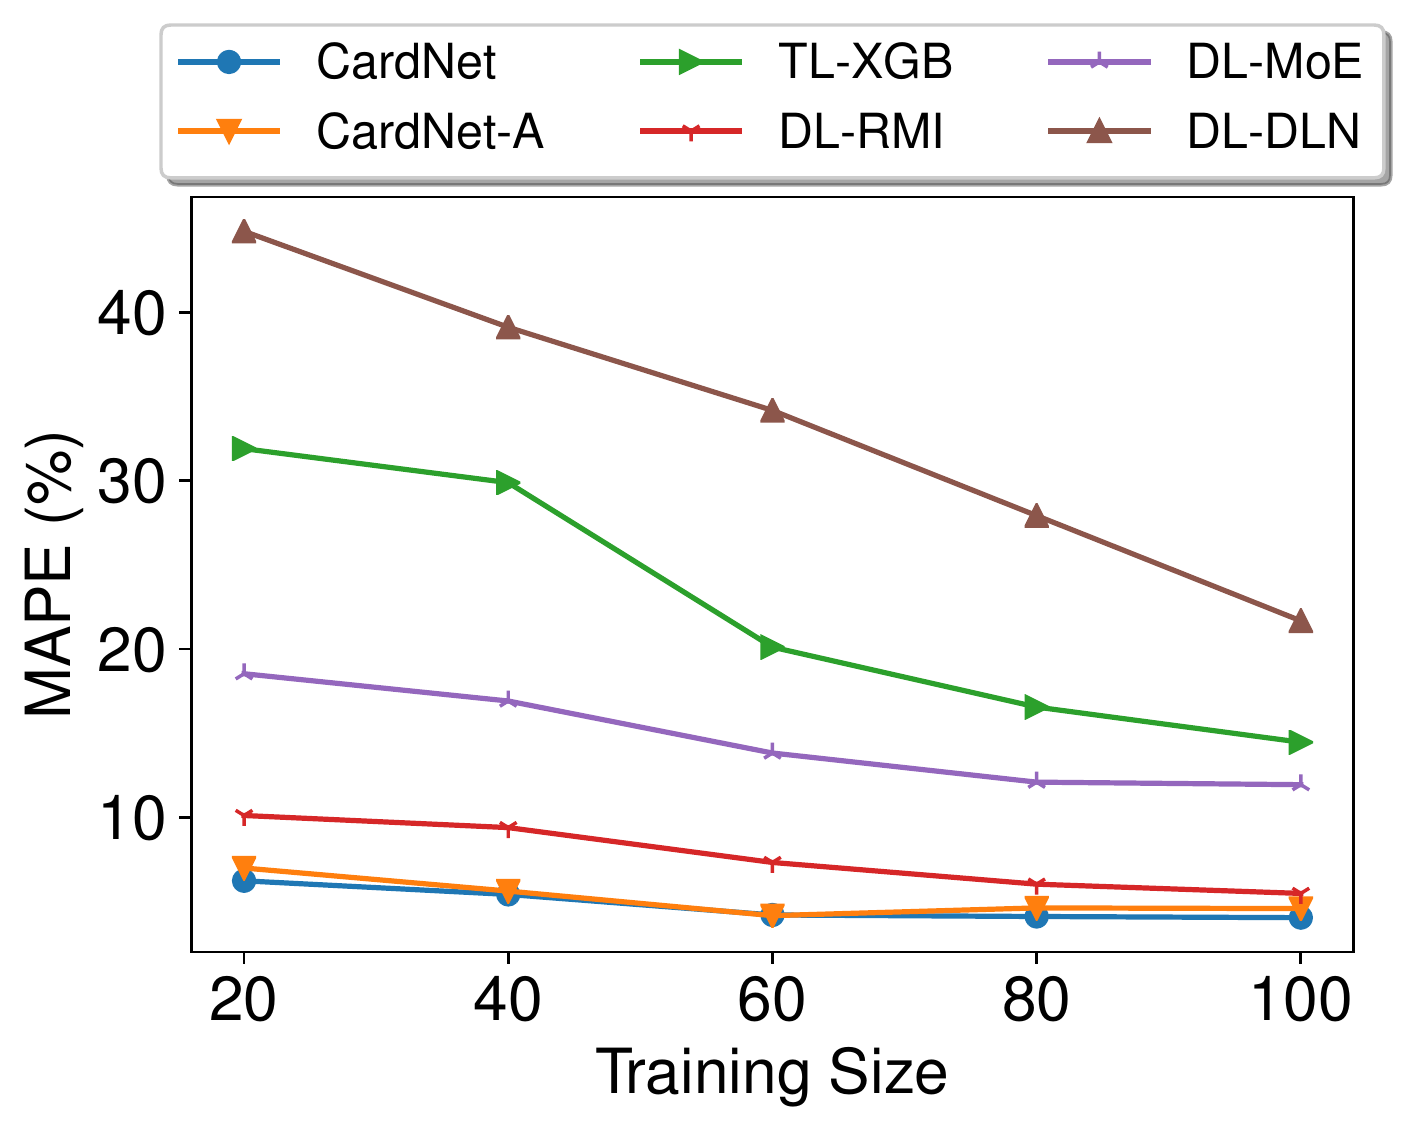}
    \label{fig:exp-glove-mape-trainsize}
  }  
  \caption{Accuracy v.s. Training Size}
  \label{fig:exp-trainsize}
\end{figure}

\subsubsection{Varying Epochs}
In Figure~\ref{fig:exp-epoch}, we show the training and validation errors of 
\modeltwo by varying epoch on \imagenet and \glovetwo datasets. At the first 
several epochs, \modeltwo converges quickly. At epoch 500, the learning rate 
is decreasing, which leads to further deceasing training and validation errors. 
After epoch 700, \modeltwo tends to be stable.

\begin{figure} [t]
  \centering
  \subfigure[\textsf{MSE}]{
    \includegraphics[width=0.46\linewidth]{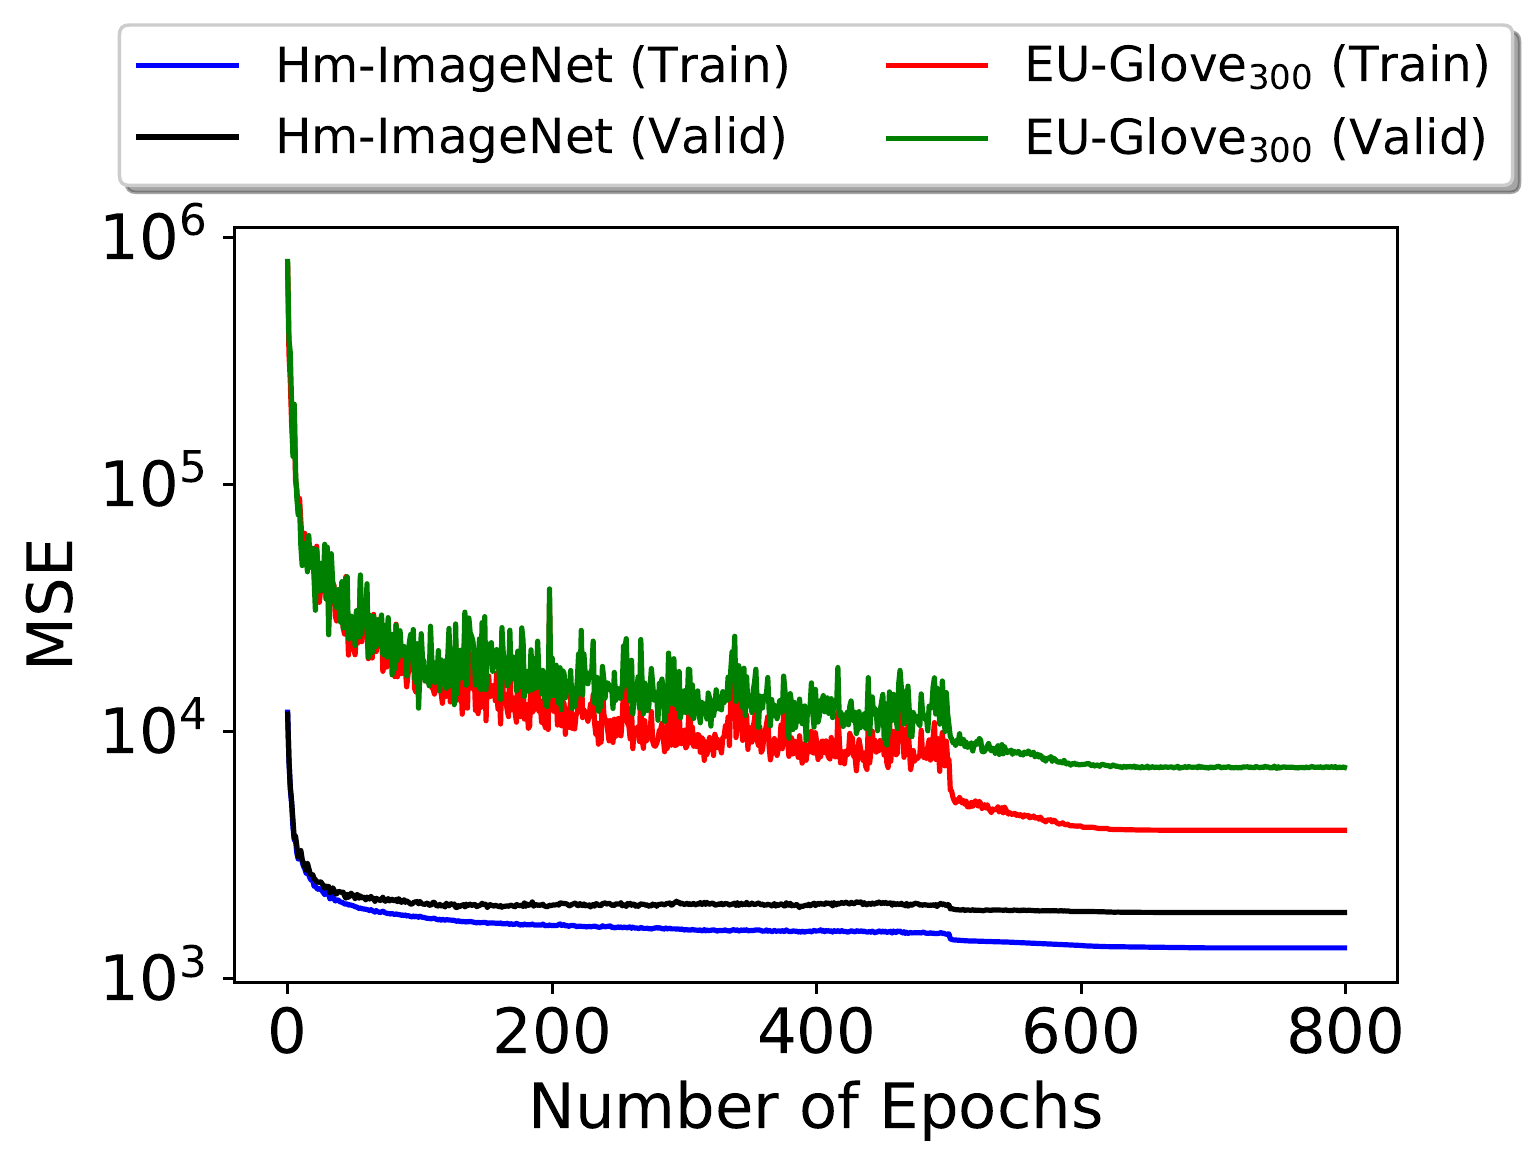}
    \label{fig:exp-epoch-mse-improve}
  }
  \subfigure[\textsf{MAPE}]{
    \includegraphics[width=0.46\linewidth]{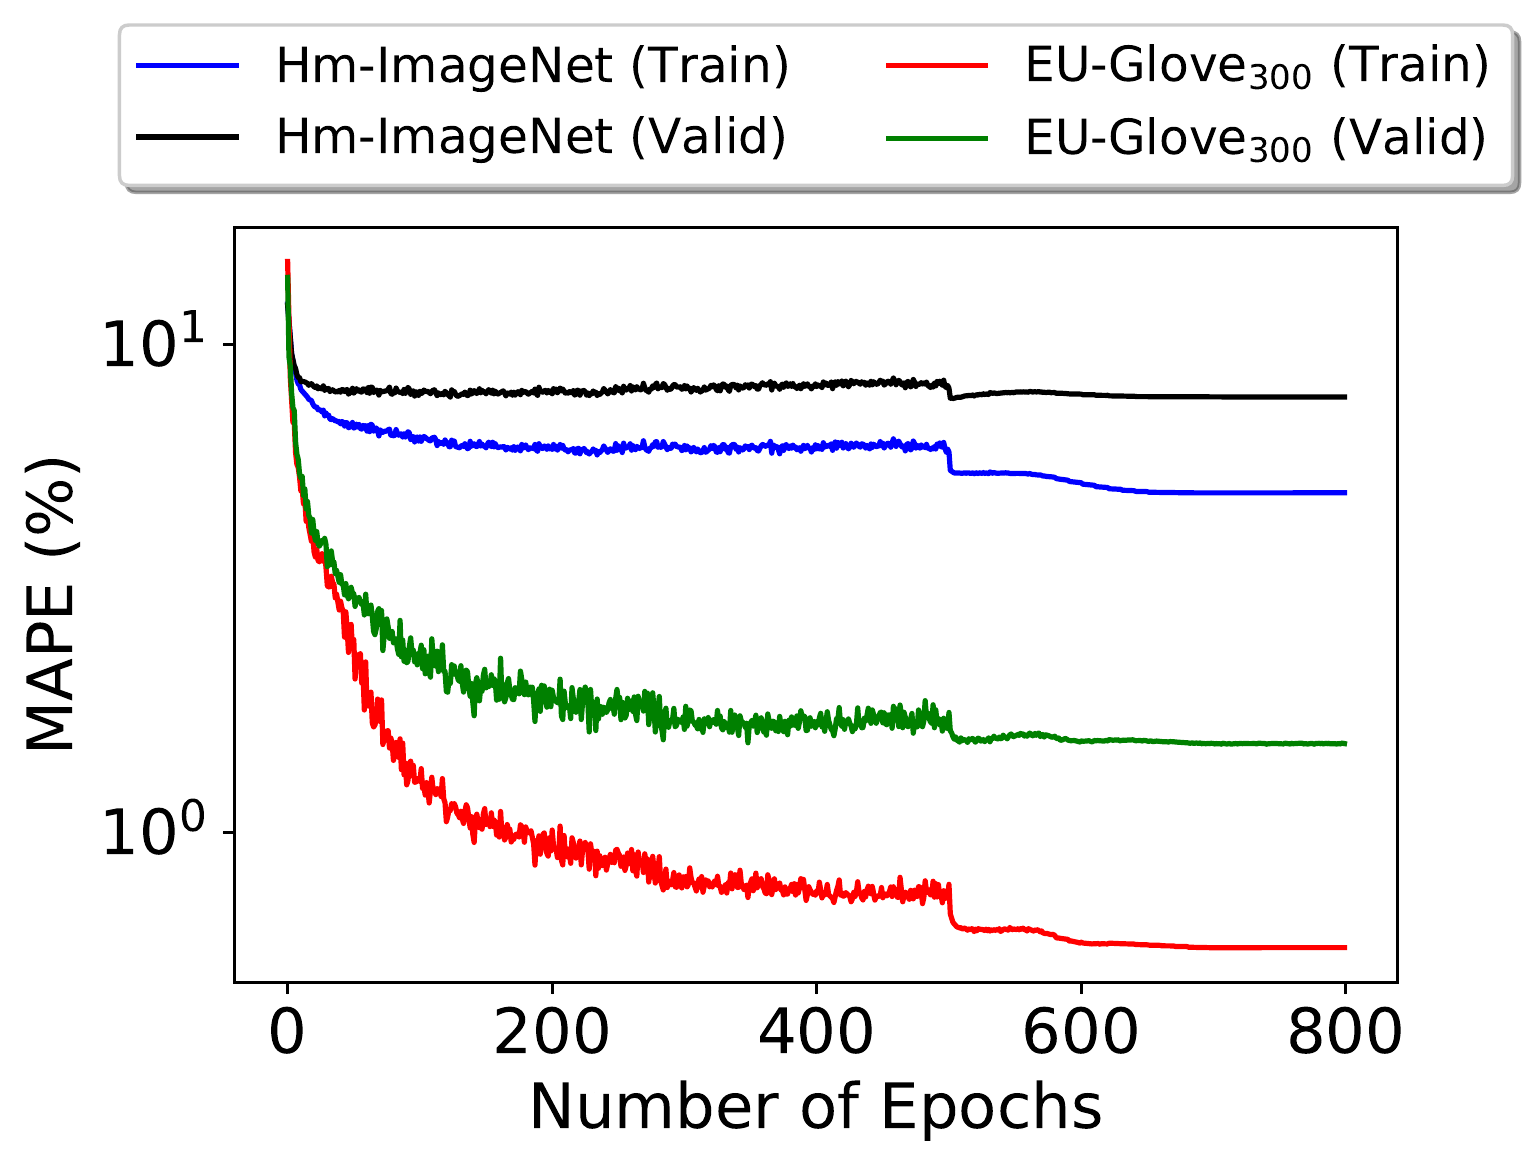}
    \label{fig:exp-epoch-mape-improve}
  }
    \caption{Training and validation errors v.s. epochs.}
  \label{fig:exp-epoch}
\end{figure}

\begin{figure} [t]
  \centering
  \subfigure[\textsf{MSE}, \gistlarge]{
    \includegraphics[width=0.46\linewidth]{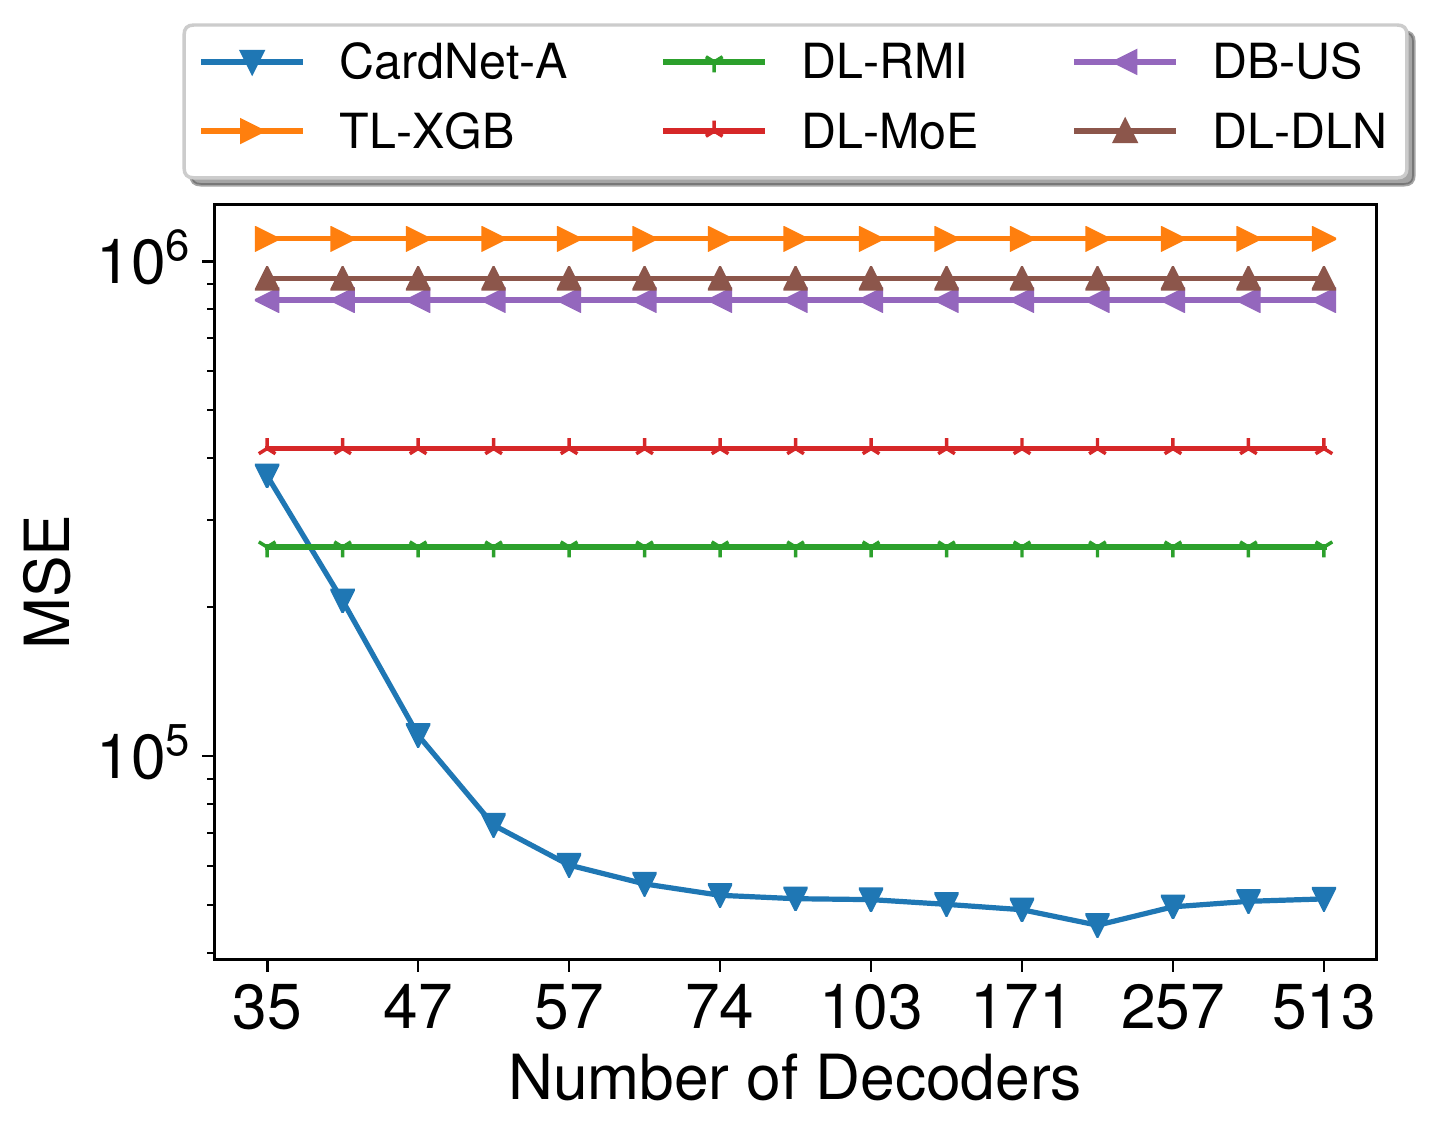}
    \label{fig:exp-granu-mse-gist}
  }
  \subfigure[\textsf{MAPE}, \gistlarge]{
    \includegraphics[width=0.46\linewidth]{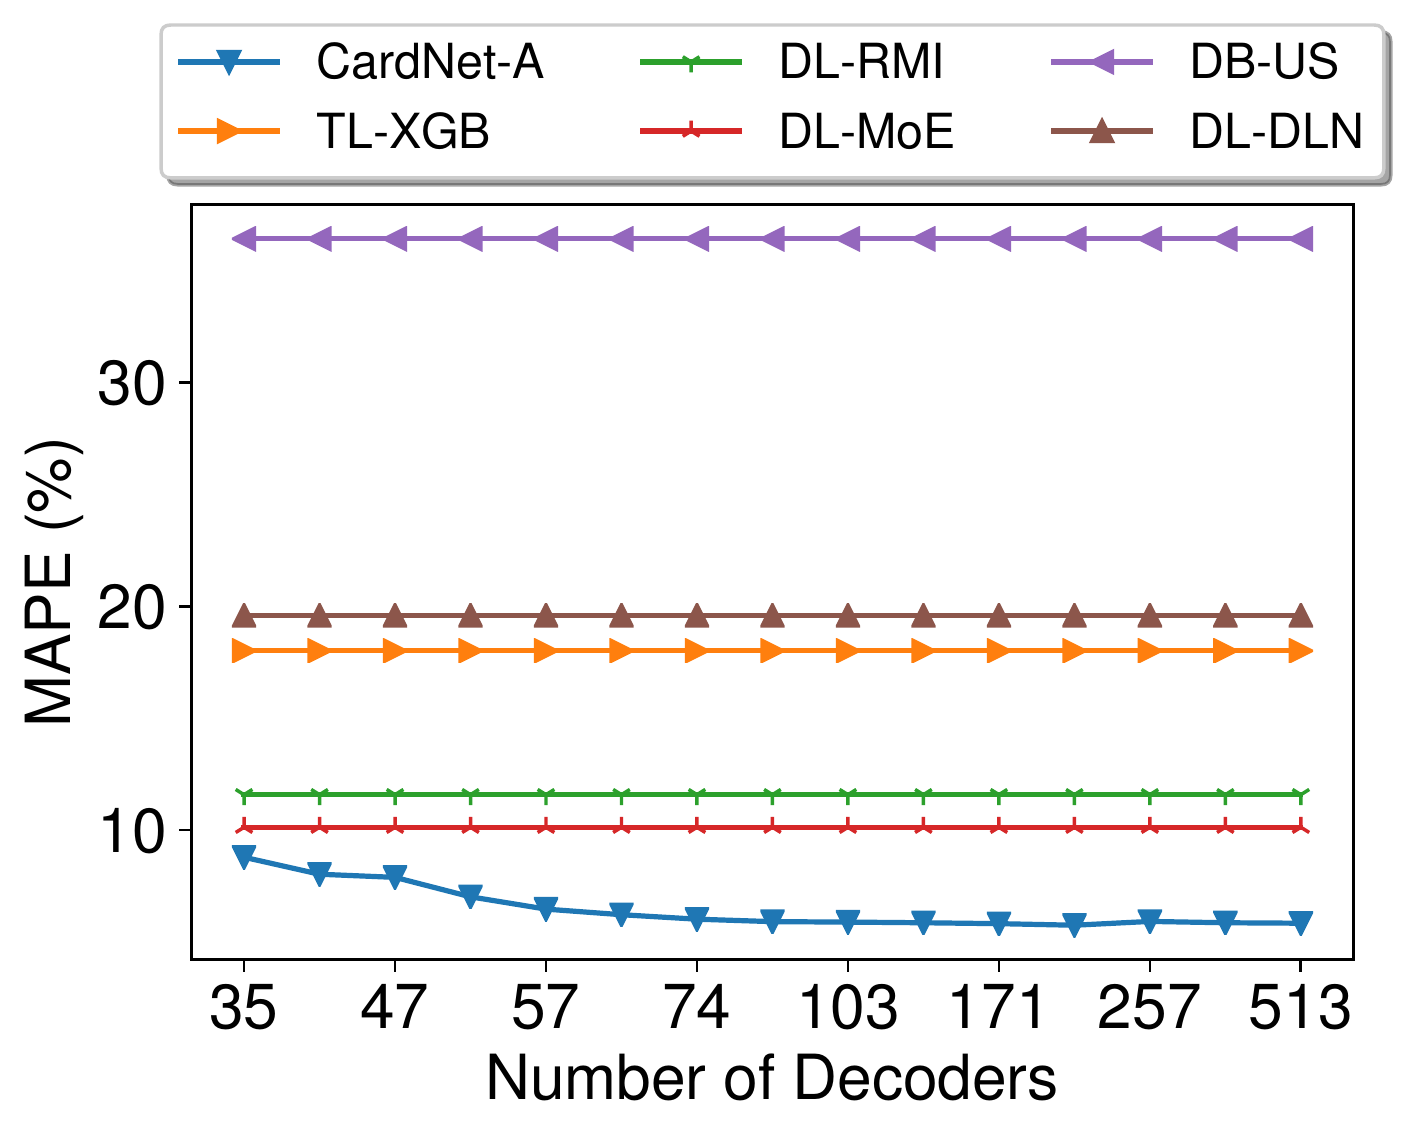}
    \label{fig:exp-granu-mape-gist}
  }
  \subfigure[\textsf{MSE}, \dblped]{
    \includegraphics[width=0.46\linewidth]{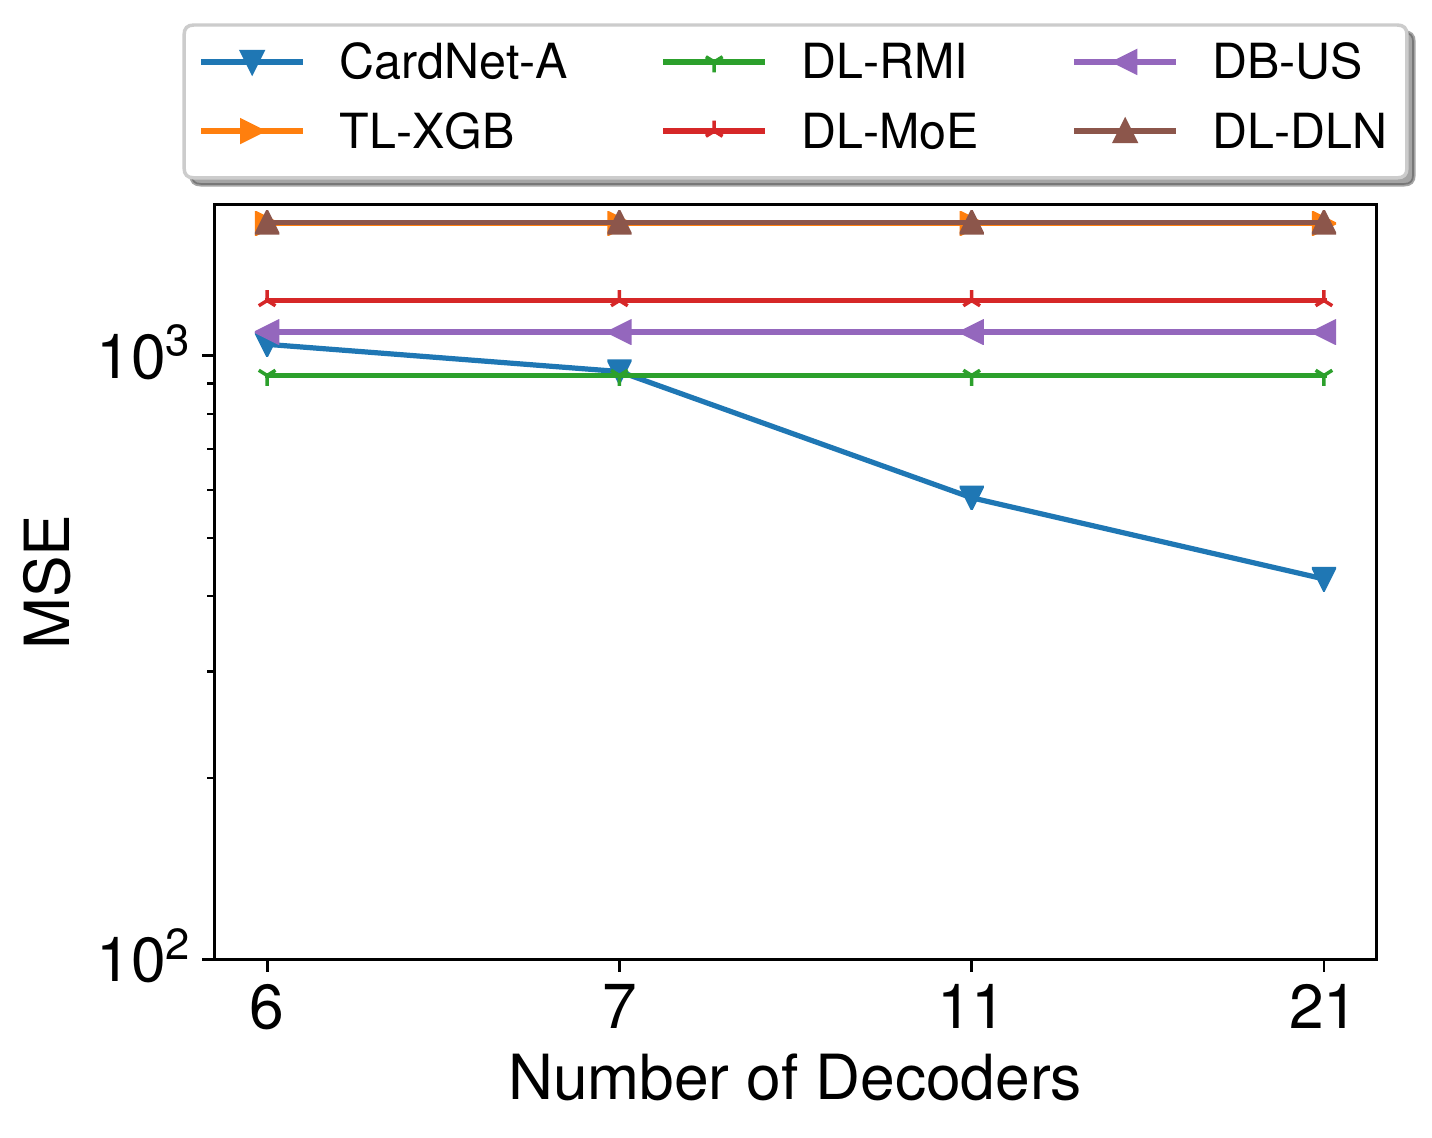}
    \label{fig:exp-granu-mse-wiki-dblped}
  }
  \subfigure[\textsf{MAPE}, \dblped]{
    \includegraphics[width=0.46\linewidth]{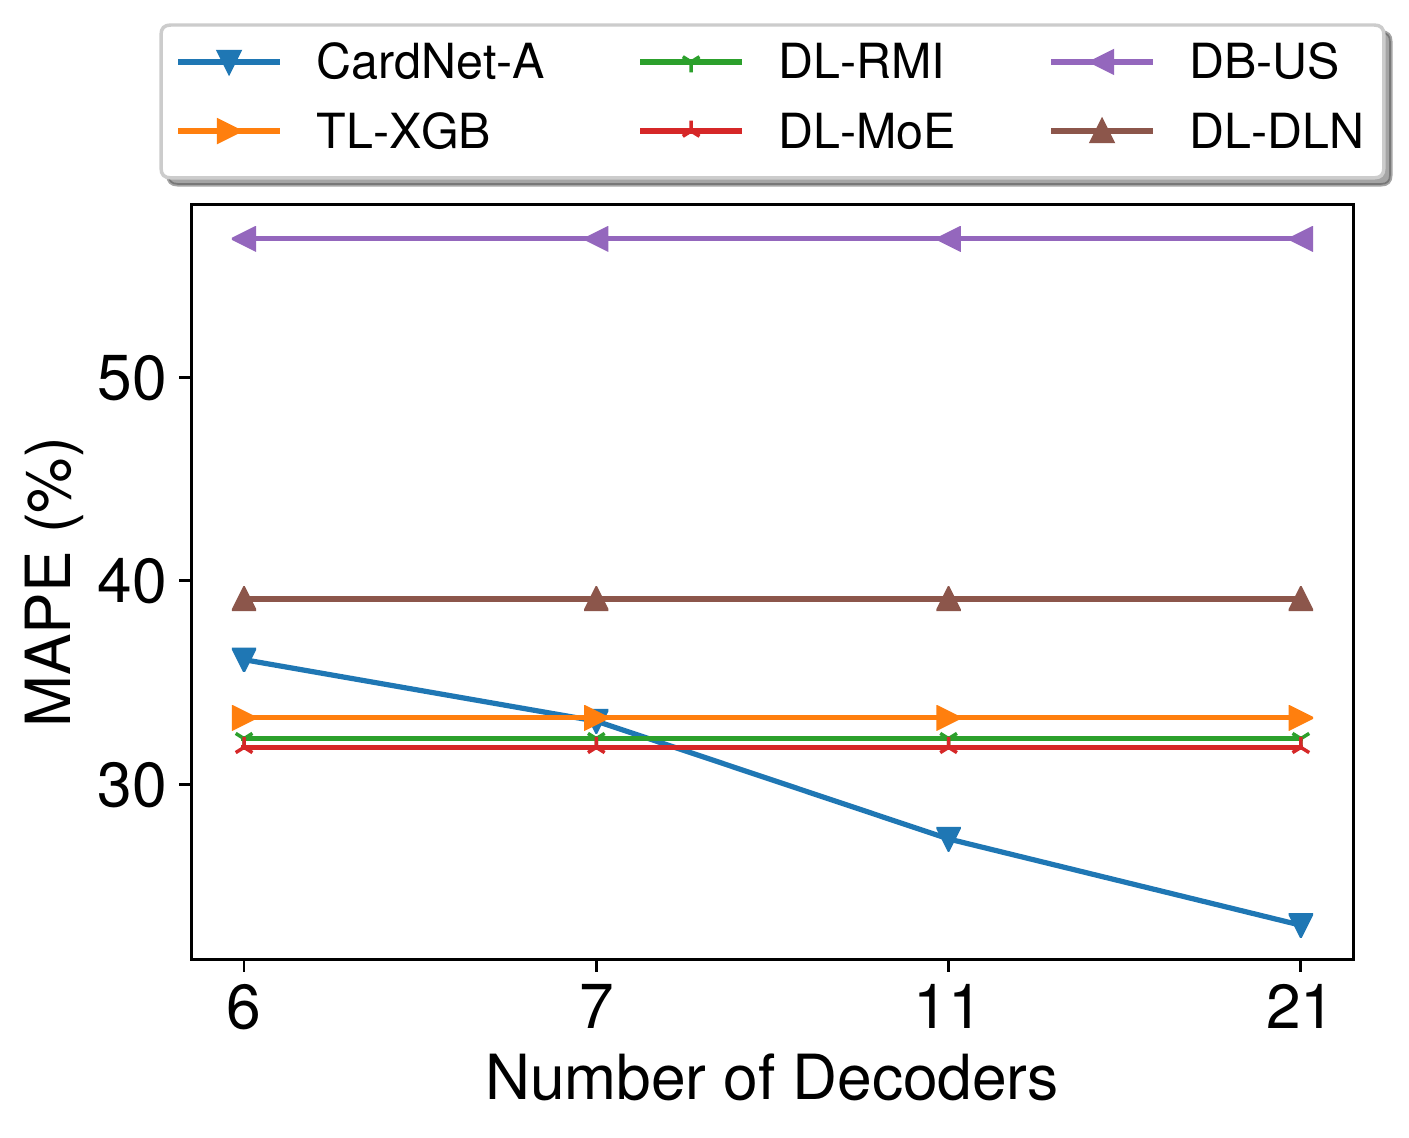}
    \label{fig:exp-granu-mape-wiki-dblped}
  }
  \subfigure[\textsf{MSE}, \wikijacc]{
    \includegraphics[width=0.46\linewidth]{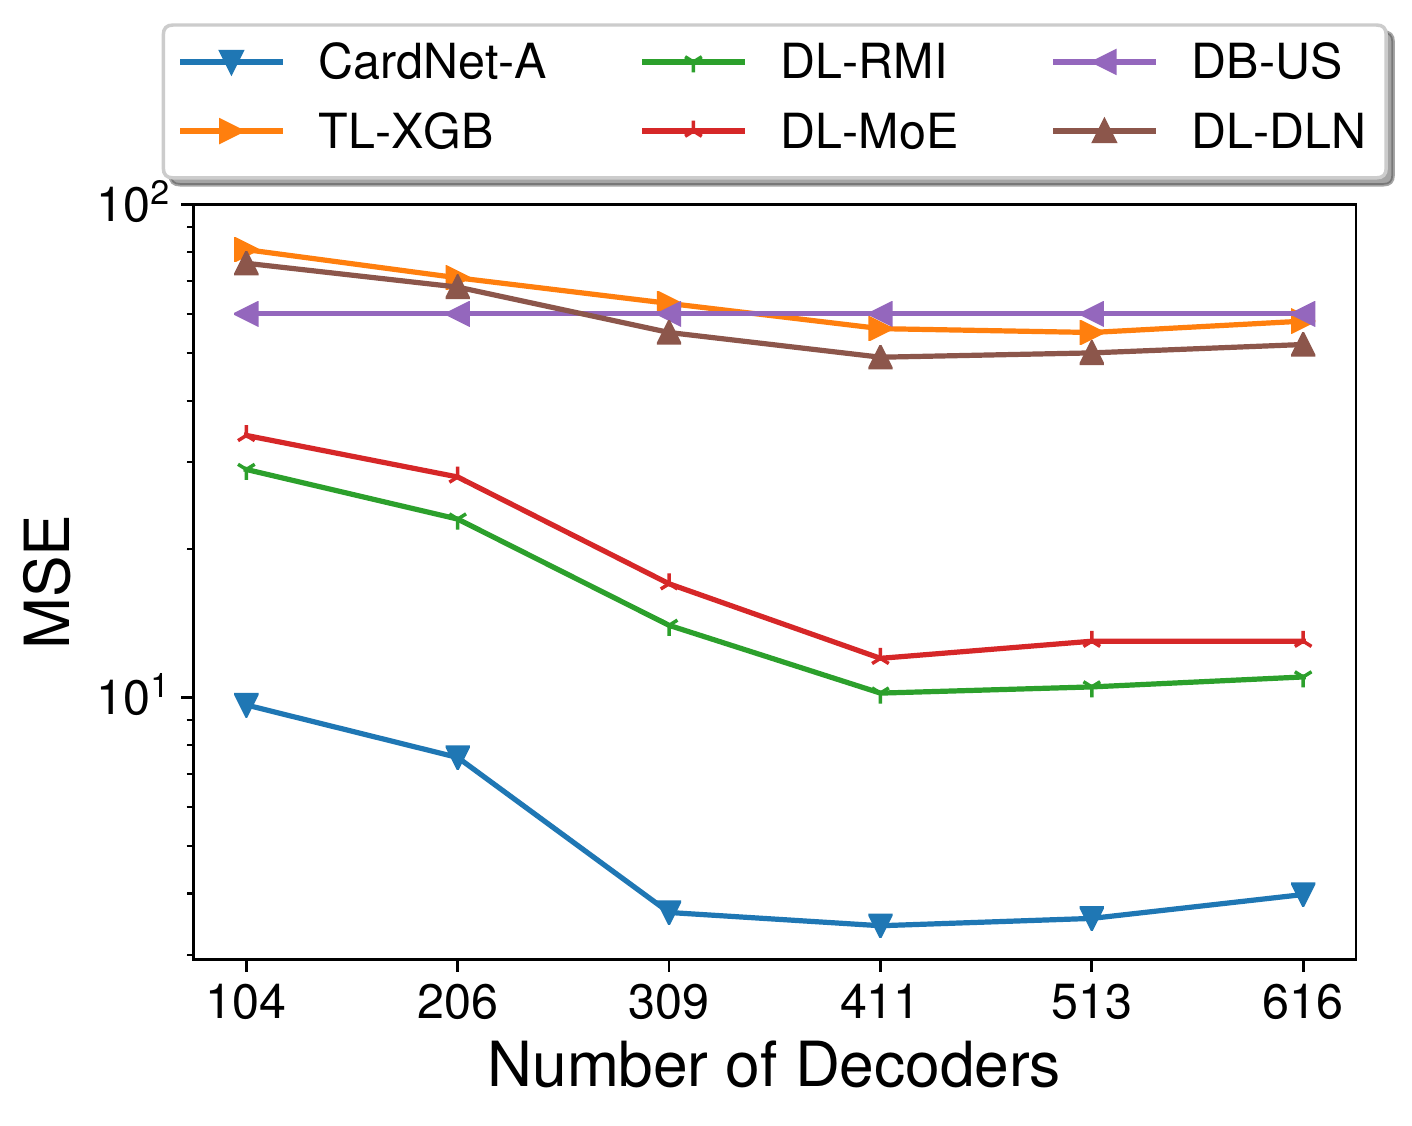}
    \label{fig:exp-granu-mse-wiki-ol}
  }
  \subfigure[\textsf{MAPE}, \wikijacc]{
    \includegraphics[width=0.46\linewidth]{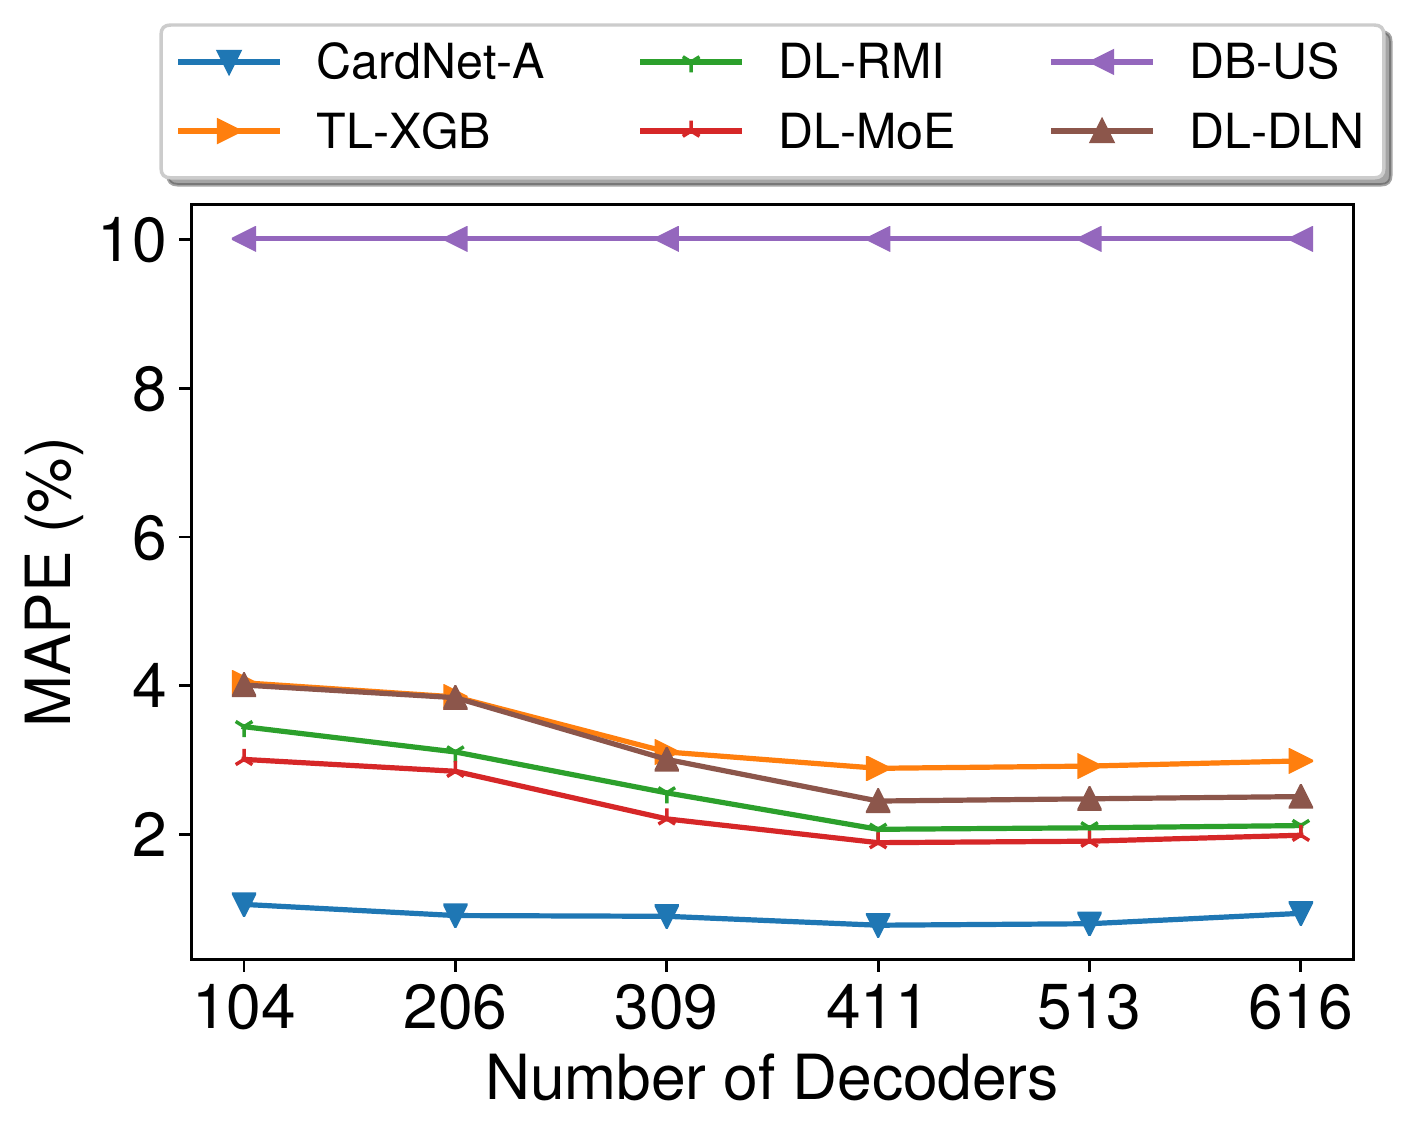}
    \label{fig:exp-granu-mape-wiki-ol}
  }
  \subfigure[\textsf{MSE}, \youtube]{
    \includegraphics[width=0.46\linewidth]{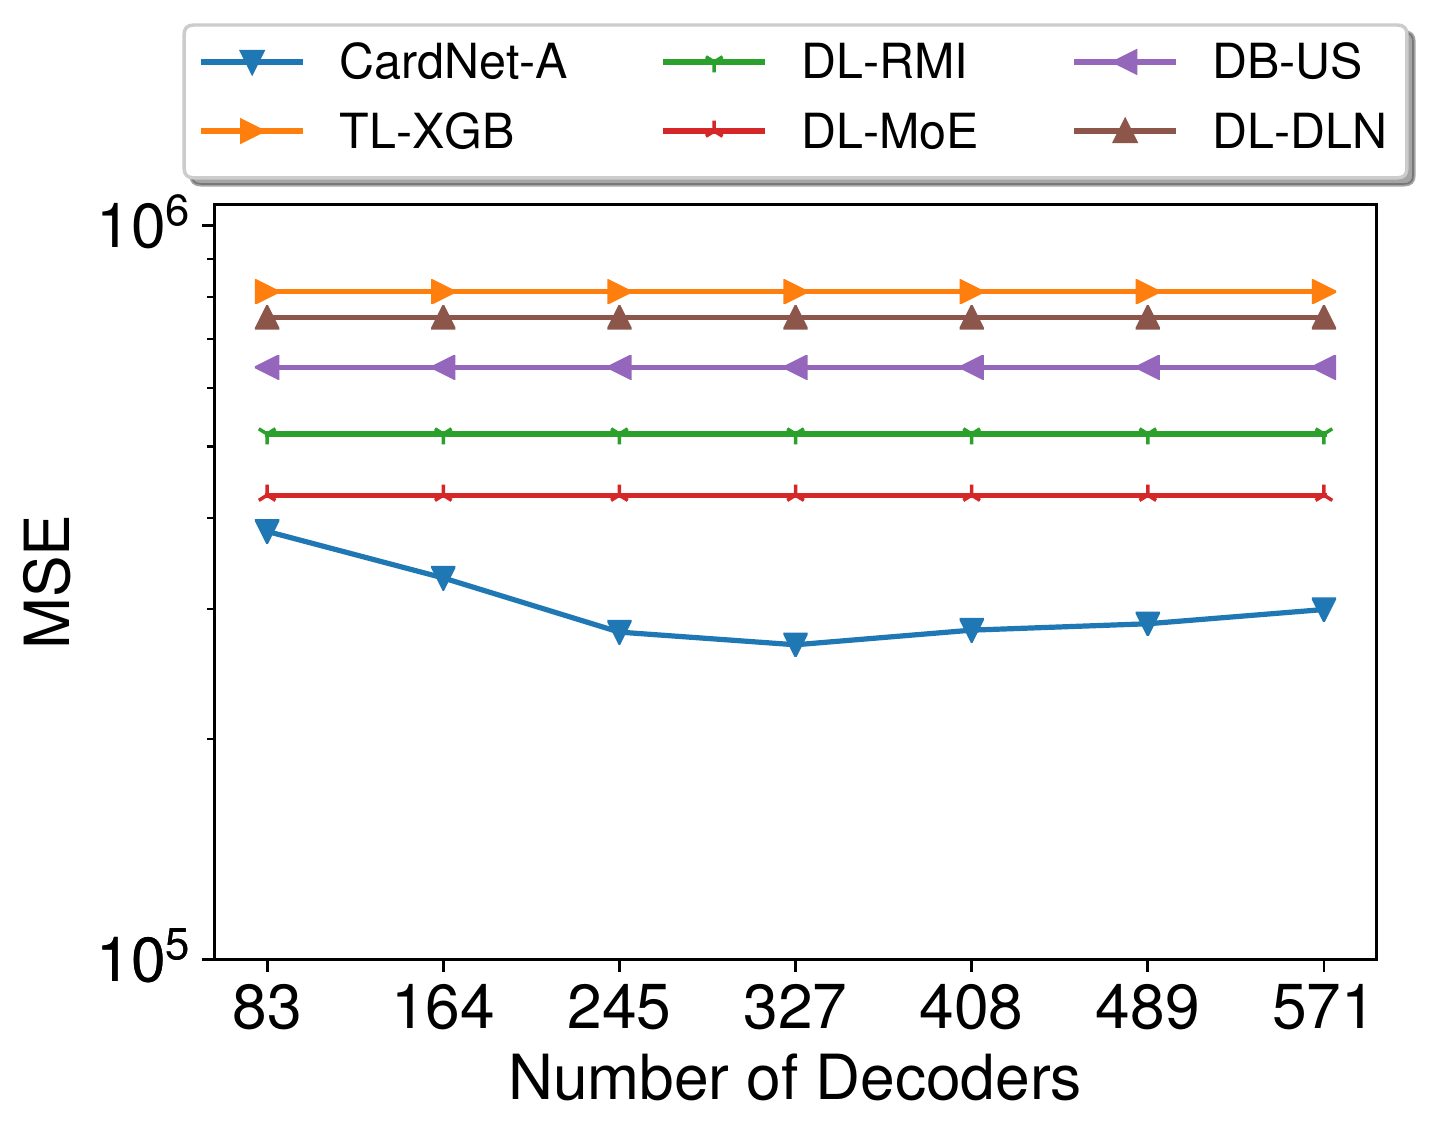}
    \label{fig:exp-granu-mse-youtube}
  }
  \subfigure[\textsf{MAPE}, \youtube]{
    \includegraphics[width=0.46\linewidth]{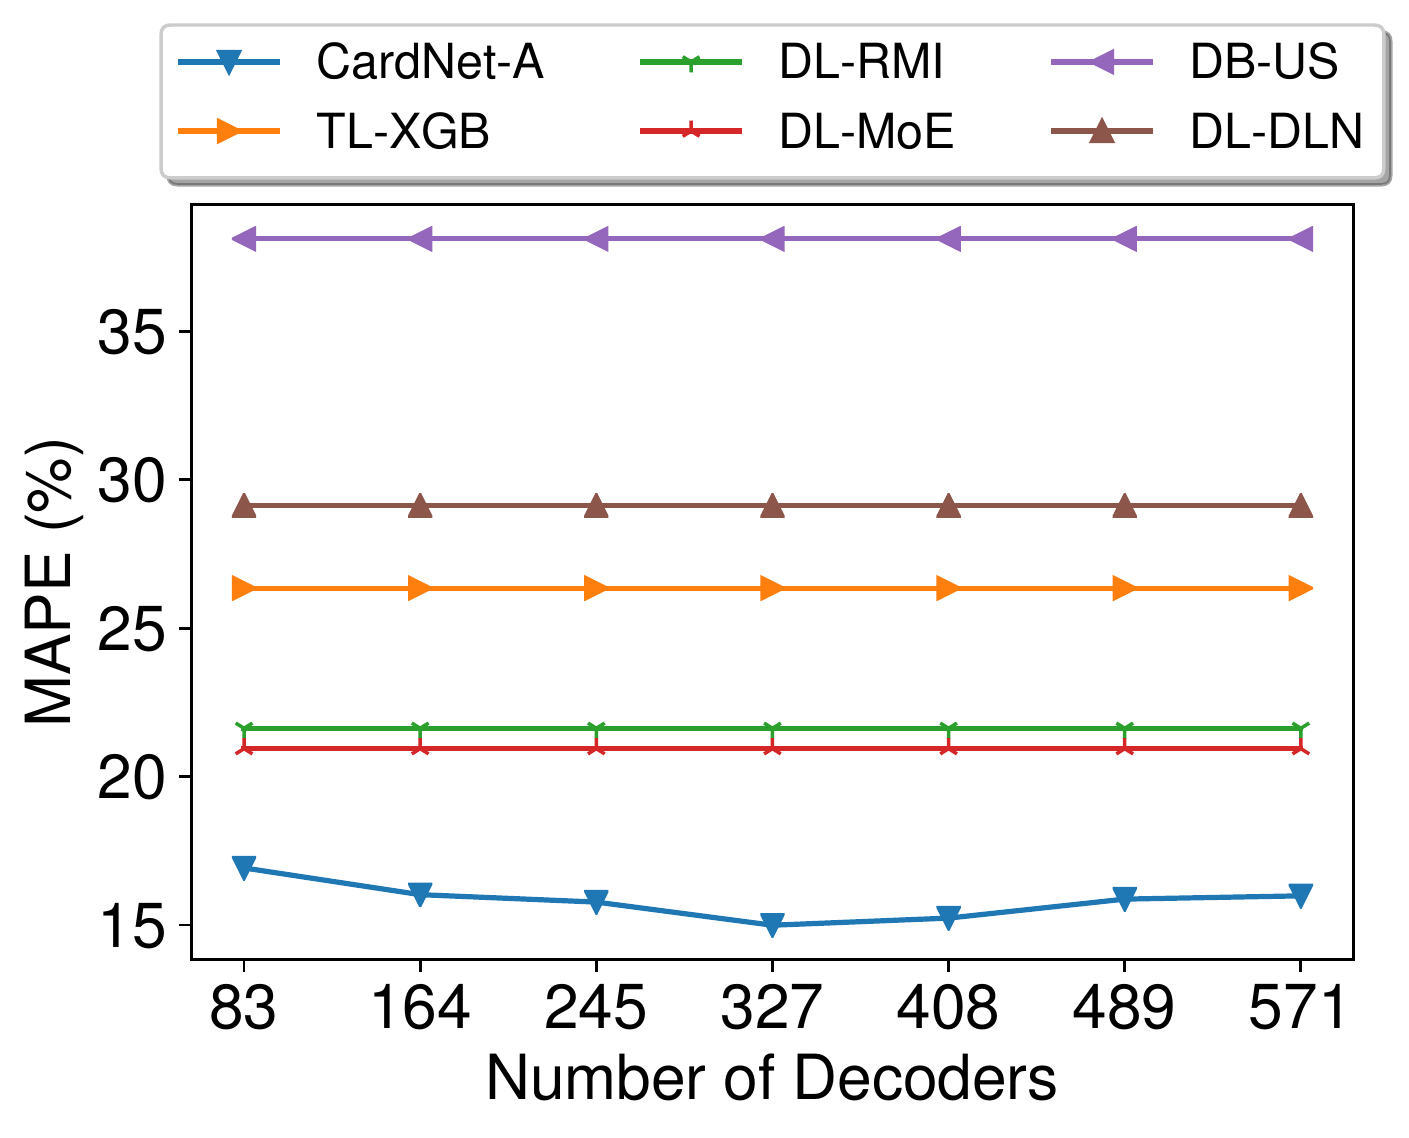}
    \label{fig:exp-granu-mape-youtube}
  }  
  \caption{Accuracy v.s. number of decoders.}
  \label{fig:exp-granu}
\end{figure}

\begin{figure} [!t]
  \centering
  \subfigure[\textsf{Time, \gistlarge}]{
    \includegraphics[width=0.46\linewidth]{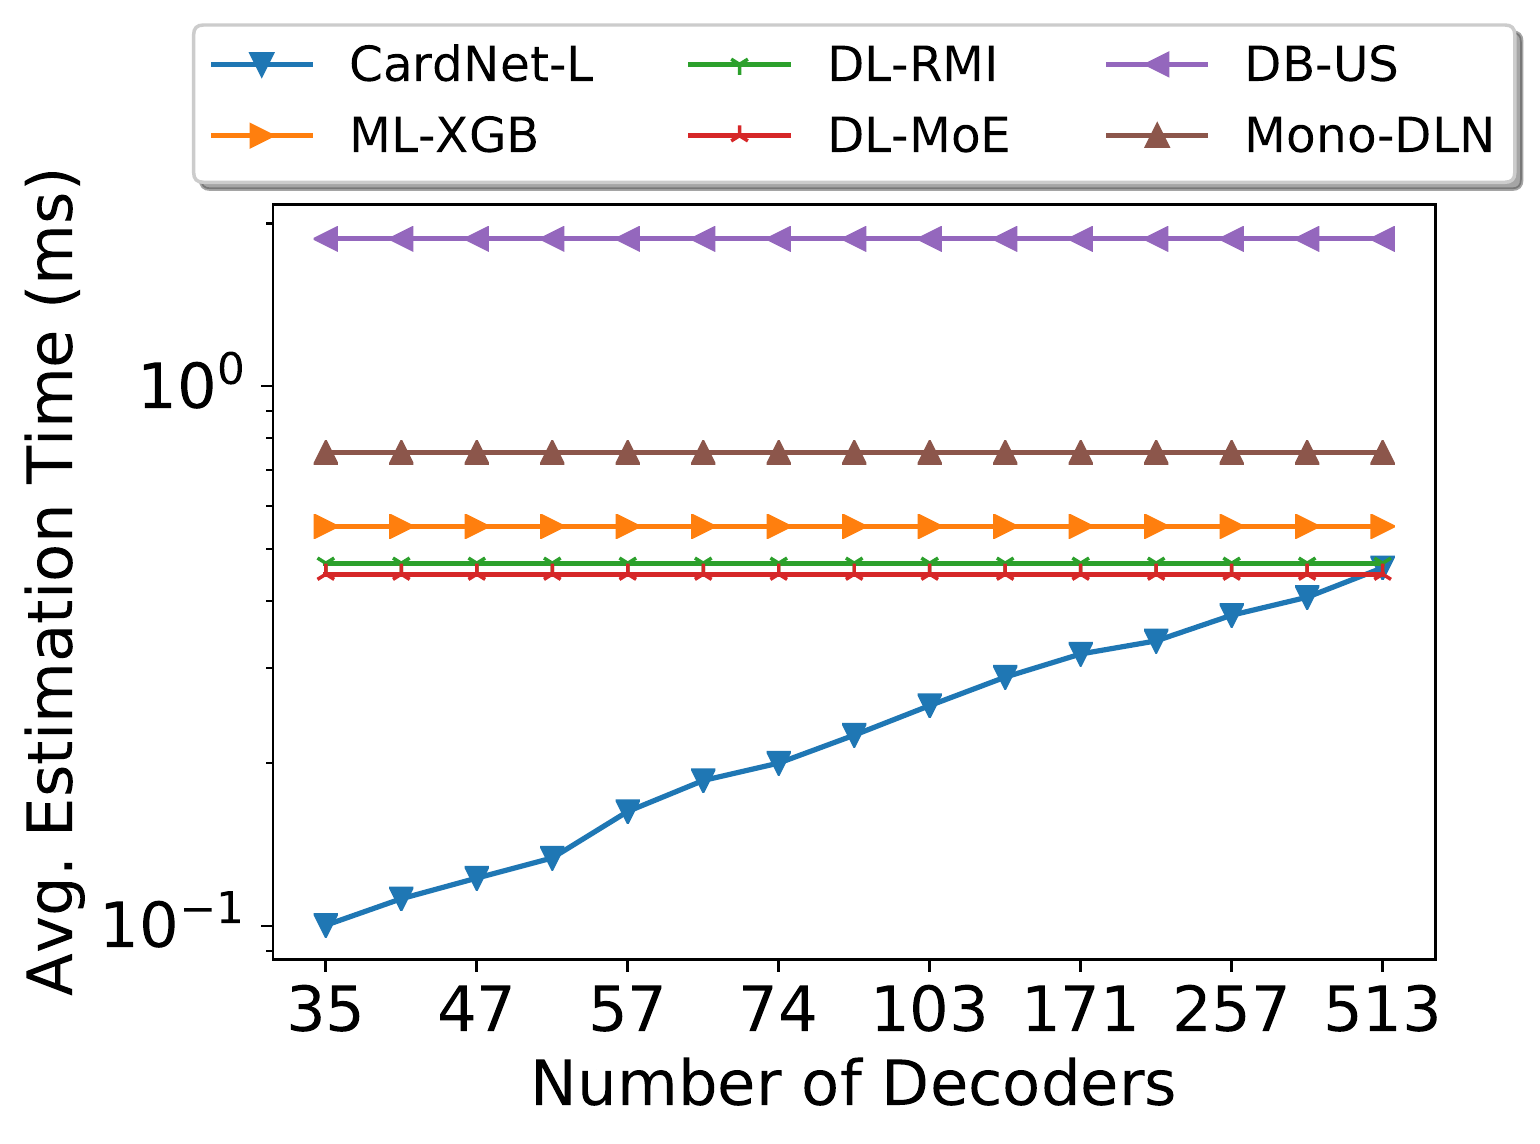}
    \label{fig:exp-granu-time-gist}
  }
  \subfigure[\textsf{Time, \dblped}]{
    \includegraphics[width=0.46\linewidth]{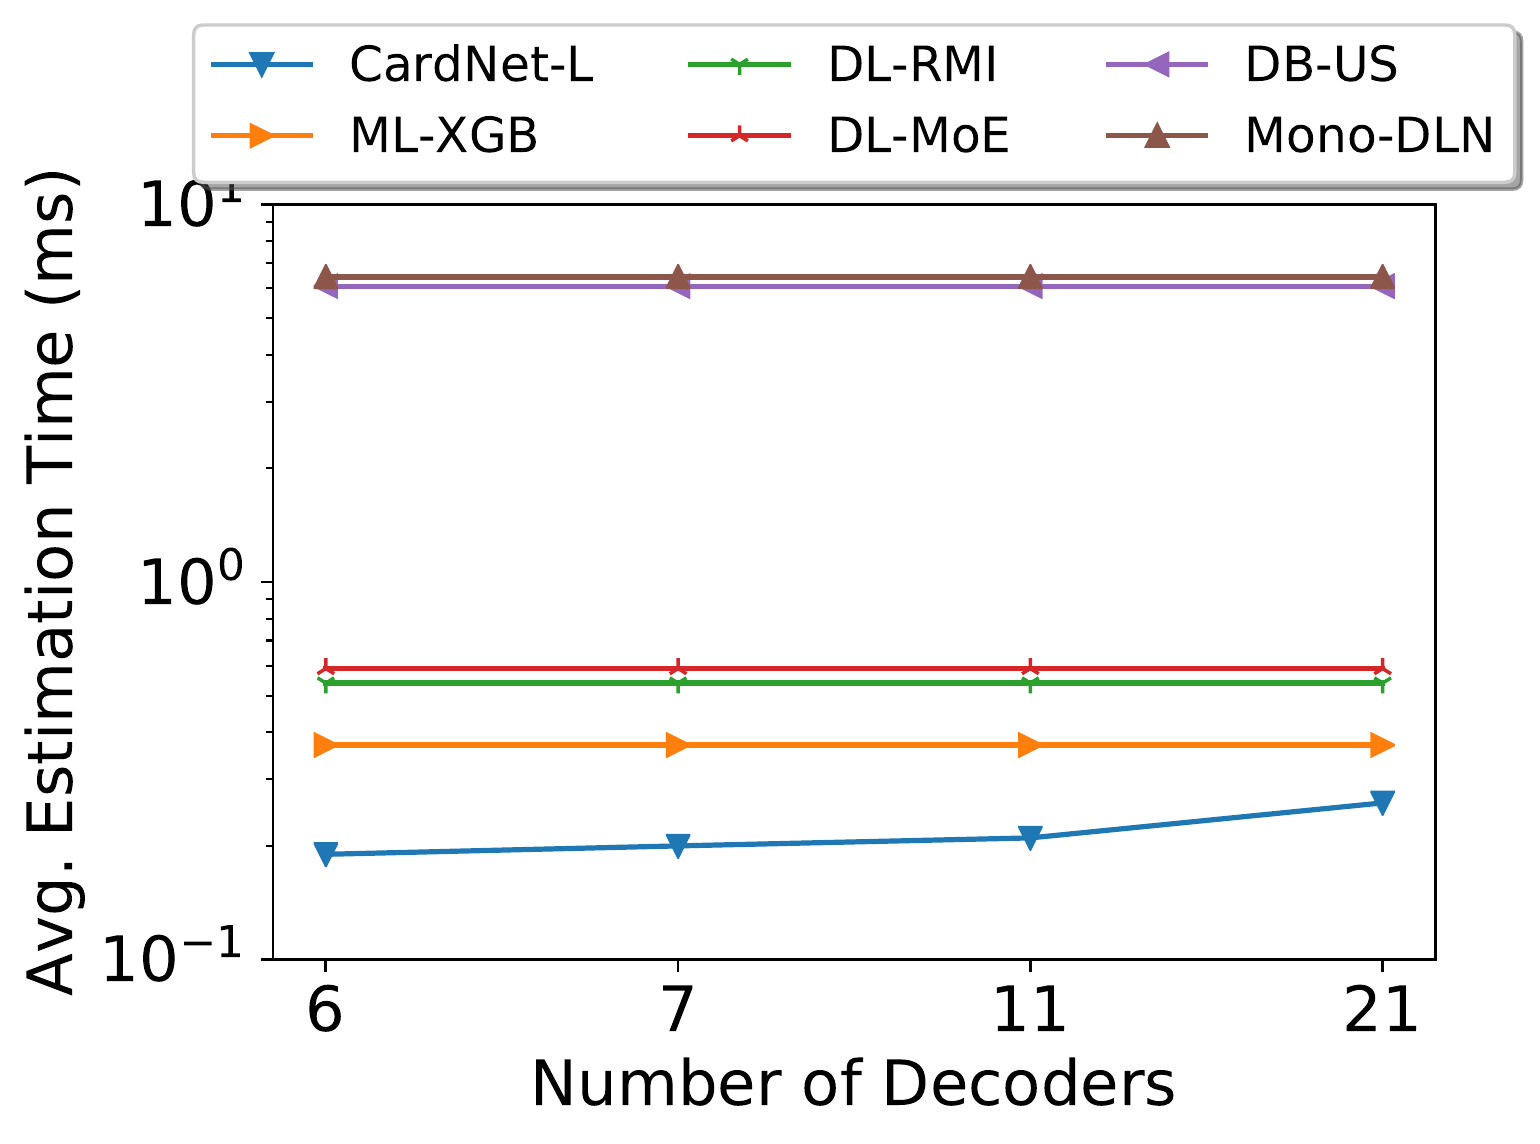}
    \label{fig:exp-granu-time-dblped}
  }
  \subfigure[\textsf{Time, \wikijacc}]{
    \includegraphics[width=0.46\linewidth]{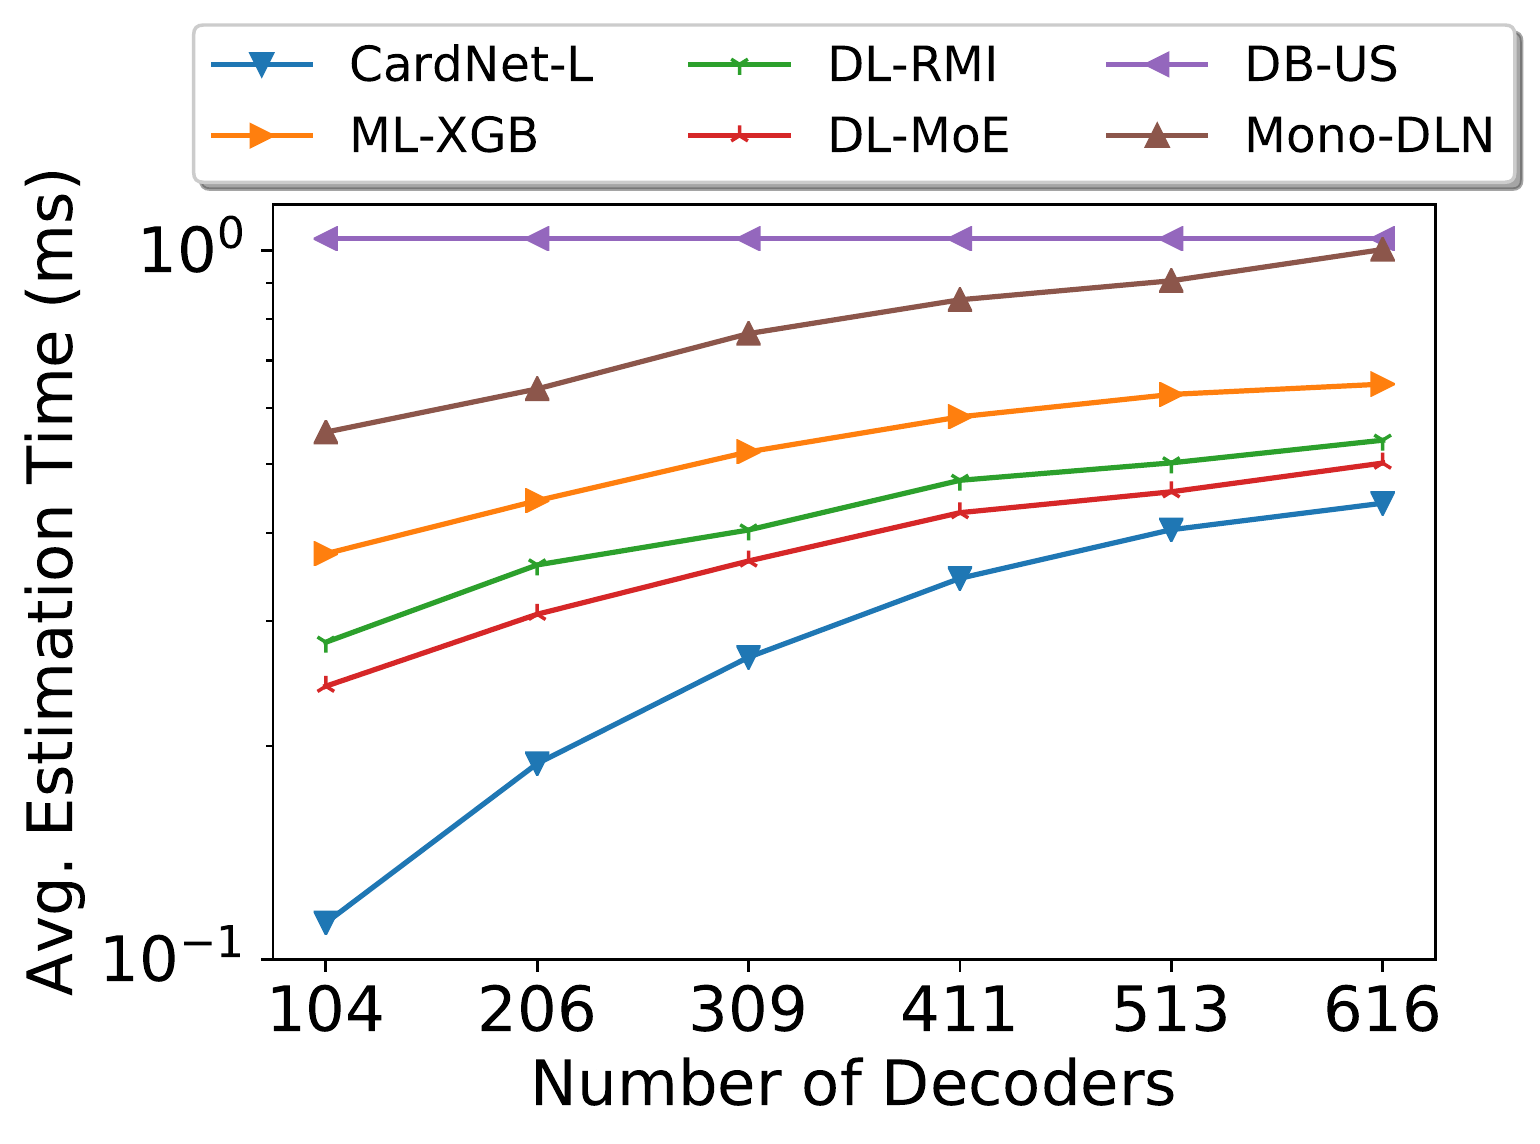}
    \label{fig:exp-granu-time-wikijacc}
  }
  \subfigure[\textsf{Time, \youtube}]{
    \includegraphics[width=0.46\linewidth]{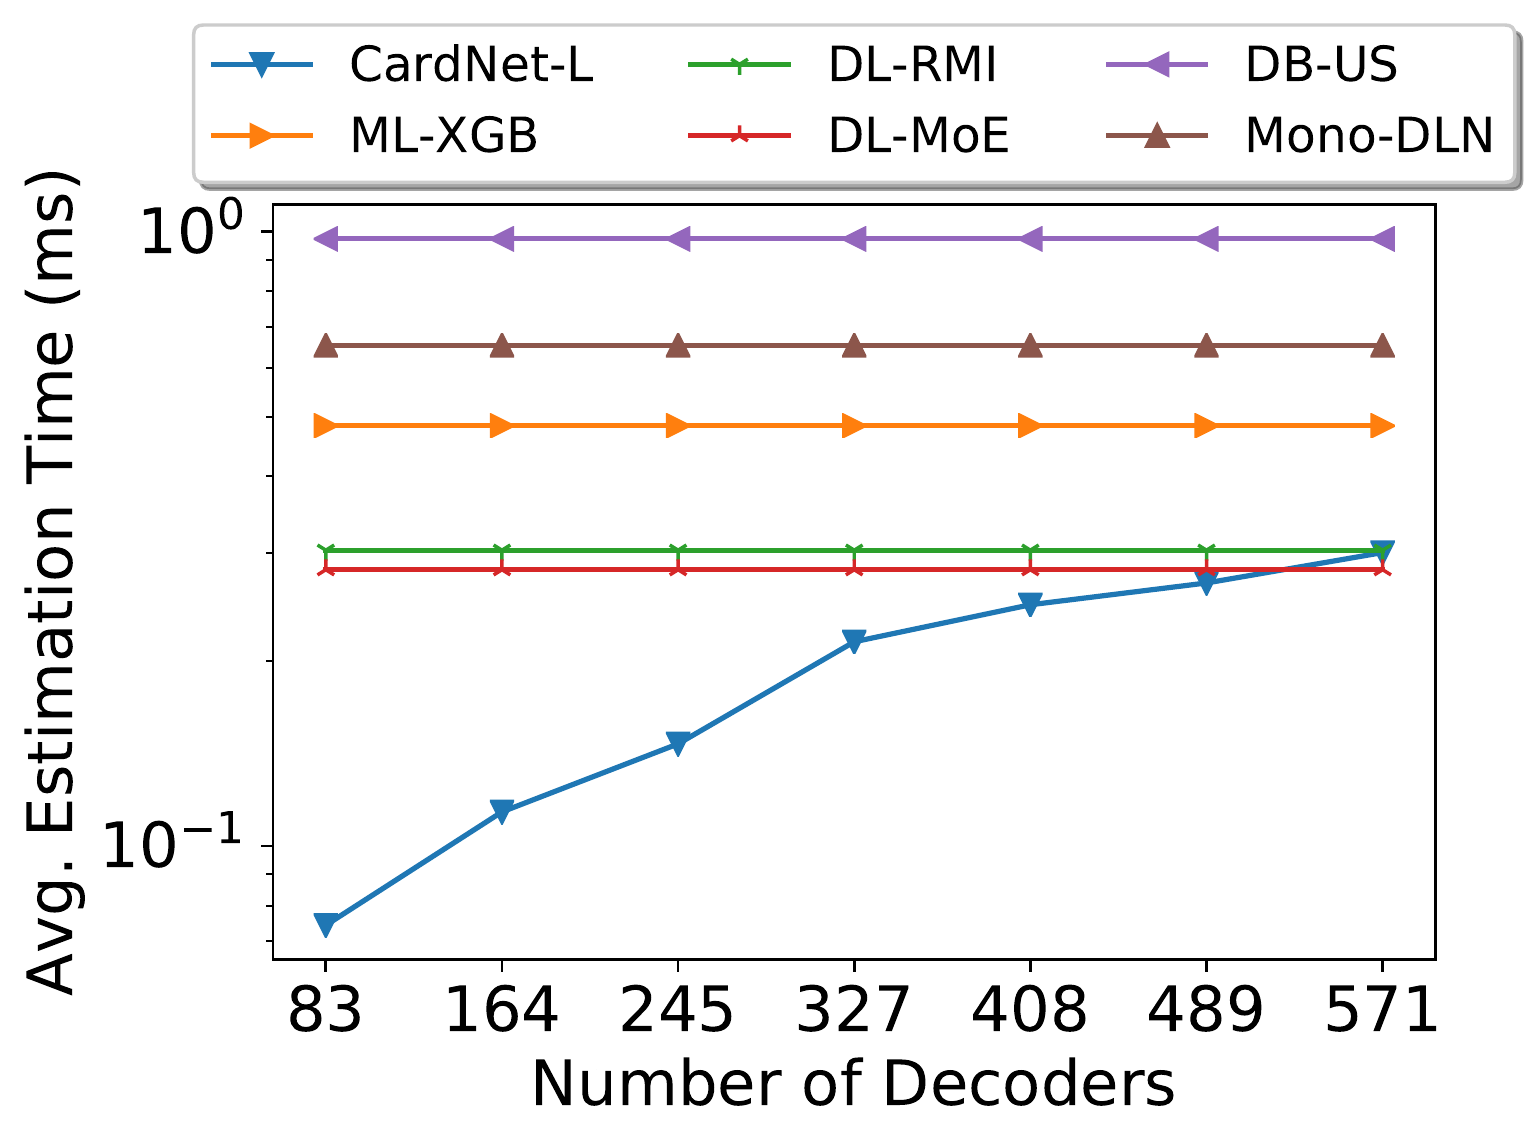}
    \label{fig:exp-granu-time-youtube}
  }  
  \caption{Estimation time v.s. number of decoders.}
  \label{fig:exp-time-granu}
\end{figure}

%\begin{savenotes}
\begin{table*} [t]
  \small%\scriptsize
  \caption{Statistics of datasets with high dimensionality.}
  \label{tab:largedataset}
  \centering
  \begin{tabular}[b]{| l | c | c | c | c | c | c | c | c | c |}
    \hline%
    \texttt{Dataset} & \texttt{Source} & \texttt{Process} & \texttt{Data Type} &
    \texttt{Domain} & \texttt{\# Records}& $\ell_{max}$ & $\ell_{avg}$ &
      \texttt{Distance} & $\theta_{max}$ \\
    \hline%
    \gistlarge & \cite{URL:gist} %\footnote{\scriptsize \url{http://horatio.cs.nyu.edu/mit/tiny/data/index.html}}~\cite{torralba200880}
    & spectral hashing~\cite{weiss2009spectral}
    & binary vector & image & 982,677 & 2048 & 2048 & Hamming & 512 \\
    \hline%
%   \wikioverlap & \textsf{Wikipedia} & 3-gram & vector & abstract & 1,150,842 & 732 & 496.06
%   & Overlap & 200 \\
%   \hline%
    \wikijacc & \cite{URL:wikipedia} %\footnote{\scriptsize \url{https://wiki.dbpedia.org/services-resources/documentation/datasets#}}~\cite{DBLP:conf/edbt/MattigFBS18} 
    & 3-gram & set & article abstract & 1,150,842 & 732 & 496.06
    & Jaccard & 0.4 \\
    \hline%
    \youtube & \cite{URL:youtube-faces} %\footnote{ \scriptsize \url{http://www.cs.tau.ac.il/~wolf/ytfaces/index.html}}~\cite{wolf2011face} 
    & normalize 
    & real-valued vector & video & 346,194 & 1770 & 1770 & Euclidean & 0.8 \\ 
    \hline%   
  \end{tabular}
\end{table*}
%\end{savenotes}

\subsection{Effect of Number of Decoders} \label{sec:exp-number-decoder}
We evaluate the effect of the number of decoders ($\tau_{\max} + 1$). 
In order to show the trend in the high dimensional case, besides \dblped, 
we use three datasets with higher dimensionality or size ($l_{avg}$ and $l_{max}$) 
than those in the other experiments. The statistics is given in Table~\ref{tab:largedataset}. 
For the three datasets, we use 512, 256, and 256 nodes for the hidden layers of 
\vae, and 1024 nodes for the first hidden layer of $\Phi$ and $\Phi'$. 
% To prevent records of small lengths from 
% affecting the granularity experiments, we remove strings in the \textsf{Abstract} 
% dataset whose lengths are smaller than 400, and generate \textsf{JC-Abstract}.

The accuracy by varying the number of decoders is shown in Figure~\ref{fig:exp-granu}. 
We also plot the results for the better ones out of each category of existing metohds. 
As seen from the results, we observe that using the largest $\tau_{\max}$ setting 
does not always lead to the best performance. E.g., on \youtube, the best 
performance is achieved at 327 decoders.When $\tau_{max}$ is small, the feature 
extraction becomes lossy and cannot successfully capture the semantics of the 
original distance function. As $\tau_{max}$ increases, the feature extraction 
becomes effective to capture the semantics. On the other hand, the performance 
drops if we set an excessively large $\tau_{max}$. This is because given a query, 
the cardinality only increases at a few thresholds (e.g., two thresholds, $\theta$ 
and $\theta + 1$, might produce the same cardinality). Using too many decoders will 
involve too many non-increasing points, posing difficulty in learning the 
regression model.~\findme{Please plot \modelone in the figures.} 
On Jaccard distance, the accuracies of existing methods also change with 
the number of decoders, because we use our feature extraction on them, which is sensitive 
to $\tau_{\max}$ for Jaccard distance. 
% E.g., on \gistlarge, a granularity of value 4 
% has the best performance with aspects of \mse and \mape. When the number
% of decoders increases to a constant value, the granularity is already
% thin enough. In this case, the larger number
% of decoders instead add more difficulties for training our model. 
% The performance starts to decrease when the granularity is relatively thick,
% For example, hashing to 512-dimensional integer vectors of \youtube and smaller
% dimensions tend to have rapidly worse performance.
% In \gistlarge, the curve of 
% 11 or larger values of granularities of \gistlarge start to increase quickly.
% The experimental results fully indicate moderate number of decoders
% in the case of large $\tau_{max}$ and high dimensions
% is enough for our model to perform well. 

In Figure~\ref{fig:exp-time-granu}, we show the average estimation time by varying 
the number of decoders. The curves of \modeltwo are approximately linear, suggesting 
that more decoders result in larger estimation cost for \modeltwo. This is expected, as 
it produces $(\tau_{\max} + 1)$ embeddings at a time.~\findme{Please plot \modelone 
in the figures.}
% For example, in \gistlarge dataset, \modeltwo of granularity value of 4 has 
% 0.21ms average estimation cost, and \moeexp, the best of others, is nearly 2
% times slower.
